# Supplementary material for: Separable pathway effects of semi-competing risks using multi-state models
Source: arXiv:2306.15947 source file (2024-10-08)
Supplement: Supplementary file 1 [file Supp0912.pdf]

# Supplementary Material for "Separable pathway effects of semi-competing risks using multi-state models"

Yuhao Deng, Yi Wang, Xiang Zhan and Xiao-Hua Zhou

**Abstract**

The supporting information consists of the following parts: (A) Proof of Theorem 1 on identification; (B) Proof of Lemma 1, Theorem 2 and corollaries on asymptotic properties; (C) Proof of Theorem 3 on uniform convergence; (D) Hypothesis tests for separable effects; (E) Efficient influence function in the general case; (F) Relaxing random censoring to conditionally random censoring; (G) Dismissible components conditional on time-varying covariates; (H) Additional simulation results; (I) Additional data analysis results.

## A Proof of Theorem 1 (Identification)

### A.1 Proof

We first look at $d\Lambda_1^{a_1}(t)$. By definition and random censoring,

$$\begin{aligned} d\Lambda_1^{a_1}(t) &= P(t \le T^{a_1} < t+dt \mid T^{a_1} \ge t, R^{a_1} \ge t) \\ &= P(t \le T^{a_1} < t+dt \mid T^{a_1} \ge t, R^{a_1} \ge t, C^{a_1} \ge t) \\ &= \frac{P(t \le T^{a_1} < t+dt, R^{a_1} > t, C^{a_1} \ge t)}{P(T^{a_1} \ge t, R^{a_1} \ge t, C^{a_1} \ge t)}. \end{aligned}$$

For the denominator,

$$\begin{aligned} & E\left\{\frac{I(\widetilde{T} \ge t, \widetilde{R} \ge t, A = a_1)}{P(A = a_1 \mid X)}\right\} \\ &= E\left\{\frac{I(T \ge t, R \ge t, C \ge t, A = a_1)}{P(A = a_1 \mid X)}\right\} \\ &= E\left\{\frac{I(T^{a_1} \ge t, R^{a_1} \ge t, C^{a_1} \ge t, A = a_1)}{P(A = a_1 \mid X)}\right\} \\ &= E\left[E\left\{\frac{I(T^{a_1} \ge t, R^{a_1} \ge t, C^{a_1} \ge t, A = a_1)}{P(A = a_1 \mid X)} \mid X, T^{a_1}, R^{a_1}, C^{a_1}\right\}\right] \\ &= E\left\{I(T^{a_1} \ge t, R^{a_1} \ge t, C^{a_1} \ge t)\frac{P(A = a_1 \mid X, T^{a_1}, R^{a_1}, C^{a_1})}{P(A = a_1 \mid X)}\right\} \\ &= E\left\{I(T^{a_1} \ge t, R^{a_1} \ge t, C^{a_1} \ge t)\frac{P(A = a_1 \mid X)}{P(A = a_1 \mid X)}\right\} \\ &= E\left\{I(T^{a_1} \ge t, R^{a_1} \ge t, C^{a_1} \ge t)\right\} \\ &= P(T^{a_1} \ge t, R^{a_1} \ge t, C^{a_1} \ge t). \end{aligned}$$

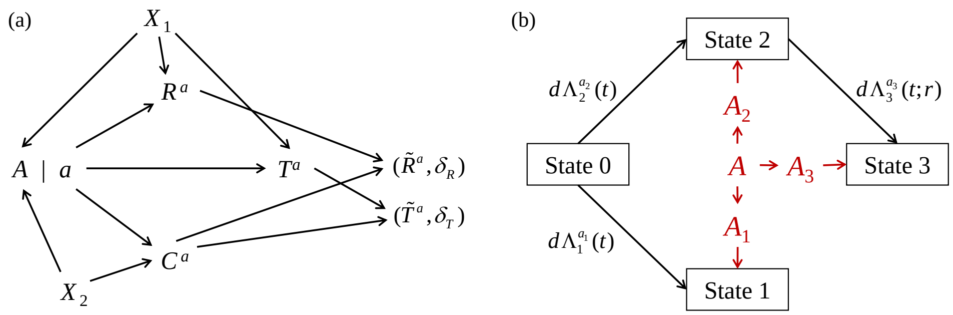


Figure S1: Multi-state model with dismissible components.

The second equation is by consistency, and the fifth equation is by ignorability. Similarly, the numerator of $d\Lambda_1^{a_1}(t)$,

$$
\begin{aligned}
& E\left\{\frac{I(t \leq \widetilde{T} < t + dt, \delta_T(1-\delta_R) = 1, A = a_1)}{P(A = a_1 \mid X)}\right\} \\
&= E\left\{\frac{I(t \leq T < t + dt, R > t, C \geq t, A = a_1)}{P(A = a_1 \mid X)}\right\} \\
&= P(t \leq T^{a_1} < t + dt, R^{a_1} > t, C^{a_1} \geq t).
\end{aligned}
$$

So

$$
d\Lambda_1^{a_1}(t) = \frac{E\{I(t \leq \widetilde{T} < t + dt, \delta_T(1-\delta_R) = 1, A = a_1)/P(A = a_1 \mid X)\}}{E\{I(\widetilde{T} \geq t, \widetilde{R} \geq t, A = a_1)/P(A = a_1 \mid X)\}}.
$$

We can show

$$
\begin{aligned}
d\Lambda_2^{a_2}(t) &= \frac{E\{I(t \leq \widetilde{R} < t + dt, \delta_R = 1 \mid A = a_2)/P(A = a_2 \mid X)P(C \geq t \mid A = a_2, X)\}}{E\{I(\widetilde{T} \geq t, \widetilde{R} \geq t, A = a_2)/P(A = a_2 \mid X)P(C \geq t \mid A = a_2, X)\}}, \\
d\Lambda_3^{a_3}(t; r) &= \frac{E\{I(t \leq \widetilde{T} < t + dt, \widetilde{R} = r, \delta_T\delta_R = 1, A = a_3)/P(A = a_3 \mid X)P(C \geq t \mid A = a_3, X)\}}{E\{I(\widetilde{T} \geq t, \widetilde{R} = r, \delta_R = 1, A = a_3)/P(A = a_3 \mid X)P(C \geq t \mid A = a_3, X)\}}
\end{aligned}
$$

in the same manner.

## A.2 On dismissible components: Collapsibility for additive hazards

Figure S1 shows the single-world intervention graph and multi-state model. We assume there are different subsets of covariates ($X_1$ and $X_2$) that affect the hazards of events and the hazard of censoring, so that random censoring holds. Specially, the way that $X_1$ affects $R^a$ and $T^a$ should be restricted in some way so that the dismissible components can hold (see the following). The primary outcome event is divided into a direct outcome event (State 1) and an indirect outcome event (State 3). Only one treatment component can have effect on a single transition hazard.

Let $a = (a_1, a_2, a_3)$. Suppose the hazards are additive for covariates and treatments,

$$
\begin{aligned}
d\Lambda_1^{a_1}(t; x) &= d\Lambda_1(t; x) + g_1(t; a_1)dt, \\
d\Lambda_2^{a_2}(t; x) &= d\Lambda_2(t; x) + g_2(t; a_2)dt, \\
d\Lambda_3^{a_3}(t; r, x) &= d\Lambda_3(t; r, x) + g_3(t; r, a_3)dt.
\end{aligned}
$$

We aim to show that the dismissible components at the individual level

$$d\Lambda_1^a(t;x) = d\Lambda_1^{a_1}(t;x),\ d\Lambda_2^a(t;x) = d\Lambda_2^{a_2}(t;x),\ d\Lambda_3^a(t;r,x) = d\Lambda_3^{a_3}(t;r,x)$$

can imply the dismissible components at the population level (if $a_2 = a_3$)

$$d\Lambda_1^a(t) = d\Lambda_1^{a_1}(t),\ d\Lambda_2^a(t) = d\Lambda_2^{a_2}(t),\ d\Lambda_3^a(t;r) = d\Lambda_3^{a_3}(t;r).$$

To see this, let $\mathcal{X}$ be the support of $X$ and $p(x)$ be the density of $X$,

$$\begin{aligned}
d\Lambda_1^a(t) &= \frac{P(t \le T^a < t+dt, R^a \ge t)}{P(T^a \ge t, R^a \ge t)} \\
&= \frac{\int_{\mathcal{X}} P(t \le T^a < t+dt, R^a \ge t \mid X=x)p(x)dx}{\int_{\mathcal{X}} P(T^a \ge t, R^a \ge t \mid X=x)p(x)dx} \\
&= \frac{\int_{\mathcal{X}} \exp\{-\Lambda_1^{a_1}(t;x) - \Lambda_2^{a_2}(t;x)\} d\Lambda_1^{a_1}(t;x)p(x)dx}{\int_{\mathcal{X}} \exp\{-\Lambda_1^{a_1}(t;x) - \Lambda_2^{a_2}(t;x)\}p(x)dx} \\
&= \frac{\int_{\mathcal{X}} \exp\{-\Lambda_1(t;x) - g_1(t;a_1) - \Lambda_2(t;x) - g_2(t;a_2)\}\{d\Lambda_1(t;x) + g_1(t;a_1)\}p(x)dx}{\int_{\mathcal{X}} \exp\{-\Lambda_1(t;x) - g_1(t;a_1) - \Lambda_2(t;x) - g_2(t;a_2)\}p(x)dx} \\
&= \frac{\int_{\mathcal{X}} \exp\{-\Lambda_1(t;x) - \Lambda_2(t;x)\}\{d\Lambda_1(t;x) + g_1(t;a_1)dt\}p(x)dx}{\int_{\mathcal{X}} \exp\{-\Lambda_1(t;x) - \Lambda_2(t;x)\}p(x)dx} \\
&= \frac{\int_{\mathcal{X}} \exp\{-\Lambda_1(t;x) - \Lambda_2(t;x)\} d\Lambda_1(t;x)p(x)dx}{\int_{\mathcal{X}} \exp\{-\Lambda_1(t;x) - \Lambda_2(t;x)\}p(x)dx} + g_1(t;a_1)dt \\
&= d\Lambda_1^*(t) + g_1(t;a_1)dt,
\end{aligned}$$

where $d\Lambda_1^*(t)$ is a quantity irrelevant to $(a_1, a_2, a_3)$, so $d\Lambda_1^a(t)$ only relies on $a_1$.

$$\begin{aligned}
d\Lambda_2^a(t) &= \frac{P(t \le R^a < t+dt, T^a \ge t)}{P(T^a \ge t, R^a \ge t)} \\
&= \frac{\int_{\mathcal{X}} P(t \le R^a < t+dt, T^a \ge t \mid X=x)p(x)dx}{\int_{\mathcal{X}} P(T^a \ge t, R^a \ge t \mid X=x)p(x)dx} \\
&= \frac{\int_{\mathcal{X}} \exp\{-\Lambda_1^{a_1}(t;x) - \Lambda_2^{a_2}(t;x)\} d\Lambda_2^{a_2}(t;x)p(x)dx}{\int_{\mathcal{X}} \exp\{-\Lambda_1^{a_1}(t;x) - \Lambda_2^{a_2}(t;x)\}p(x)dx} \\
&= \frac{\int_{\mathcal{X}} \exp\{-\Lambda_1(t;x) - g_1(t;a_1) - \Lambda_2(t;x) - g_2(t;a_2)\}\{d\Lambda_2(t;x) + g_2(t;a_2)\}p(x)dx}{\int_{\mathcal{X}} \exp\{-\Lambda_1(t;x) - g_1(t;a_1) - \Lambda_2(t;x) - g_2(t;a_2)\}p(x)dx} \\
&= \frac{\int_{\mathcal{X}} \exp\{-\Lambda_1(t;x) - \Lambda_2(t;x)\}\{d\Lambda_2(t;x) + g_2(t;a_2)dt\}p(x)dx}{\int_{\mathcal{X}} \exp\{-\Lambda_1(t;x) - \Lambda_2(t;x)\}p(x)dx} \\
&= \frac{\int_{\mathcal{X}} \exp\{-\Lambda_1(t;x) - \Lambda_2(t;x)\} d\Lambda_2(t;x)p(x)dx}{\int_{\mathcal{X}} \exp\{-\Lambda_1(t;x) - \Lambda_2(t;x)\}p(x)dx} + g_2(t;a_2)dt \\
&= d\Lambda_2^*(t) + g_2(t;a_2)dt,
\end{aligned}$$

where $d\Lambda_2^*(t)$ is a quantity irrelevant to $(a_1, a_2, a_3)$, so $d\Lambda_2^a(t)$ only relies on $a_2$.

$$\begin{aligned}
d\Lambda_3^a(t;r) &= \frac{P(t \le T^a < t+dt, R^a = r)}{P(T^a \ge t, R^a = r)} \\
&= \frac{\int_{\mathcal{X}} P(t \le T^a < t+dt \mid R^a = r, X=x)P(R^a = r \mid X=x)p(x)dx}{\int_{\mathcal{X}} P(T^a \ge t \mid R^a = r, X=x)P(R^a = r \mid X=x)p(x)dx}
\end{aligned}$$

$$
\begin{aligned}
&= \frac{\int_{\mathcal{X}} \exp\{-\Lambda_3^{a_3}(t;r,x)\} d\Lambda_3^{a_3}(t;r,x) \exp\{-\Lambda_1^{a_1}(r;x) - \Lambda_2^{a_2}(r;x)\}\lambda_2^{a_2}(r;x)p(x)dx}{\int_{\mathcal{X}} \exp\{-\Lambda_3^{a_3}(t;r,x)\} \exp\{-\Lambda_1^{a_1}(r;x) - \Lambda_2^{a_2}(r;x)\}\lambda_2^{a_2}(r;x)p(x)dx} \\
&= \frac{\int_{\mathcal{X}} \exp\{-\Lambda_3(t;r,x)\}\{d\Lambda_3(t;r,x) + g_3(t;r,a_3)dt\} \exp\{-\Lambda_1(r;x) - \Lambda_2(r;x)\}\{\lambda_2(r;x) + g_2(r;a_2)\}p(x)dx}{\int_{\mathcal{X}} \exp\{-\Lambda_3(t;r,x)\} \exp\{-\Lambda_1(r;x) - \Lambda_2(r;x)\}\{\lambda_2(r;x) + g_2(r;a_2)\}p(x)dx} \\
&= d\Lambda_3^*(t;r,a_2) + g_3(t;r,a_3)dt,
\end{aligned}
$$

where $d\Lambda_3^*(t;r,a_2)$ is a quantity irrelevant to $a_1$. There can be two cases where the dismissible components assymption holds. (1) If we let $a_2 = a_3$ (corresponding to $\text{SPE}_{0\to 3}(a_1)$ for any fixed $a_1$), then $d\Lambda_3^a(t;r)$ only relies on $a_2 = a_3$ but not on $a_1$. (2) If $d\Lambda_3^{a_3}(t;r,x_3)$ and $d\Lambda_2^{a_2}(x_2)$ with different subsets of covariates, then $d\Lambda_3^a(t;r) = d\Lambda_3^a(t;r,x_2) = d\Lambda_3^{a_3}(t;r,x_2) = d\Lambda_3^{a_3}(t;r)$.

# B Proof of Theorem 2 (Asymptotics)

## B.1 Lemma 1: Construction of martingales

**Lemma 1.** *Under Markov assumption $d\Lambda_3^{a_3}(t;r) = d\Lambda_{3,ma.}^{a_3}(t)$, let*

$$
\begin{aligned}
N_{3,ma.}(t;a_3) &= \sum_{i=1}^n w_i(a_3) I\{\widetilde{T}_i \le t, \delta_i^T \delta_i^R = 1\}, \\
Y_{3,ma.}(t;a_3) &= \sum_{i=1}^n w_i(a_3) I\{\widetilde{T}_i \ge t, \widetilde{R}_i \le t, \delta_i^R = 1\}, \\
Y_{3,ma.}^w(t;a_3) &= \sum_{i=1}^n w_i(a_3)^2 I\{\widetilde{T}_i \ge t, \widetilde{R}_i \le t, \delta_i^R = 1\}, \\
M_{3,ma.}(t;a_3) &= \int_0^t \left\{ dN_{3,ma.}(s;a_3) - Y_{3,ma.}(s;a_3) d\Lambda_{3,ma.}^{a_3}(s) \right\}.
\end{aligned}
$$

*Under semi-Markov assumption $d\Lambda_3^{a_3}(t;r) = d\Lambda_{3,sm.}^{a_3}(t-r)$, let*

$$
\begin{aligned}
N_{3,sm.}(u;a_3) &= \sum_{i=1}^n w_i(a_3) I\{\widetilde{T}_i - \widetilde{R}_i \le u, \delta_i^T \delta_i^R = 1\}, \\
Y_{3,sm.}(u;a_3) &= \sum_{i=1}^n w_i(a_3) I\{\widetilde{T}_i - \widetilde{R}_i \ge u, \delta_i^R = 1\}, \\
Y_{3,sm.}^w(u;a_3) &= \sum_{i=1}^n w_i(a_3)^2 I\{\widetilde{T}_i - \widetilde{R}_i \ge u, \delta_i^R = 1\}, \\
M_{3,sm.}(u;a_3) &= \int_0^u \left\{ dN_{3,sm.}(s;a_3) - Y_{3,sm.}(s;a_3) d\Lambda_{3,sm.}^{a_3}(s) \right\}.
\end{aligned}
$$

*Let $N_{3,j}(t)$, $Y_{3,j}(t)$, $Y_{3,j}^w(t)$ and $M_{3,j}(t)$ be the counting prosess, at-risk process, weighted at-risk process and residual of ther indirect outcome event ($j = ma.$ and $sm.$), whose expressions are given in Supplementary Material B.1. Then*

$$
d\Lambda_{3,j}^{a_3}(t) = E\left\{ \int_0^t \frac{dN_{3,j}(s;a_3)}{Y_{3,j}(s;a_3)} \right\}, \quad j = ma. \text{ and } sm..
$$

*The residuals $\{M_j(t;a_j) : j = 1,2,3(ma.$ and $sm.)\}$ are martingales with respect to filters*

$$
\mathcal{F}_j^{a_j}(t) = \{w_i(a_j), I(T_i^{a_j} \ge s, R_i^{a_j} \ge s, C_i^{a_j} \ge s) : s \le t, i = 1,\dots,n\}, \ j = 1,2,
$$

$$\mathcal{F}^{a_3}_{3,ma.}(t) = \{w_i(a_3), I(T_i^{a_3} \geq s, T_i^{a_3} \geq R_i^{a_3}, C_i^{a_3} \geq s) : s \leq t, i = 1, \ldots, n\},$$
$$\mathcal{F}^{a_3}_{3,sm.}(t) = \{w_i(a_3), I(T_i^{a_3} - R_i^{a_3} \geq s, C_i^{a_3} - R_i^{a_3} \geq s) : s \leq t, i = 1, \ldots, n\},$$

*with* $E\{dM_j(t;a_j) \mid \mathcal{F}^{a_j}_j(t)\} = 0$ *and* $\mathrm{var}\{dM_j(t;a_j) \mid \mathcal{F}^{a_j}_j(t)\} = Y_j^w(t;a_j)d\Lambda_j^{a_j}(t)$.

Define the counterfactual counting processes and at-risk processes for $d\Lambda_1^{a_1}(t)$ and $d\Lambda_2^{a_2}(t)$ as

$$N_{i1}(t;a_1) = I\{T_i^{a_1} \leq t, R_i^{a_1} > t, C_i^{a_1} \geq t\},\ Y_{i1}(t;a_1) = I\{T_i^{a_1} \geq t, R_i^{a_1} \geq t, C_i^{a_1} \geq t\},$$
$$N_{i2}(t;a_2) = I\{R_i^{a_2} \leq t, T_i^{a_2} \geq t, C_i^{a_1} \geq t\},\ Y_{i2}(t;a_2) = I\{T_i^{a_2} \geq t, R_i^{a_2} \geq t, C_i^{a_2} \geq t\},$$

where $i = 1, \ldots, n$. They can only take values 0 or 1. Define weights

$$w_i(a_j) = \frac{I(A_i = a_j)}{P(A_i = a_j \mid X_i)},\ j = 1, 2, 3.$$

Let the weighted counting processes and at-risk processes for $d\Lambda_1^{a_1}(t)$ and $d\Lambda_2^{a_2}(t)$ be

$$N_1(t;a_1) = \sum_{i=1}^n w_i(a_1)N_{i1}(t;a_1) = \sum_{i=1}^n \frac{1}{P(A_i = a_1 \mid X_i)} I\{\widetilde{T}_i \leq t, \delta_i^T(1-\delta_i^R) = 1, A_i = a_1\},$$
$$Y_1(t;a_1) = \sum_{i=1}^n w_i(a_1)Y_{i1}(t;a_1) = \sum_{i=1}^n \frac{1}{P(A_i = a_1 \mid X_i)} I\{\widetilde{T}_i \geq t, \widetilde{R}_i \geq t, A_i = a_1\},$$
$$N_2(t;a_2) = \sum_{i=1}^n w_i(a_2)N_{i2}(t;a_1) = \sum_{i=1}^n \frac{1}{P(A_i = a_2 \mid X_i)} I\{\widetilde{R}_i \leq t, \widetilde{T}_i \geq t, \delta_i^R = 1, A_i = a_2\},$$
$$Y_2(t;a_2) = \sum_{i=1}^n w_i(a_2)N_{i2}(t;a_2) = \sum_{i=1}^n \frac{1}{P(A_i = a_2 \mid X_i)} I\{\widetilde{T}_i \geq t, \widetilde{R}_i \geq t, A_i = a_2\}.$$

These equations mean that the counterfactual processes are identifiable. Define a filter

$$\mathcal{F}^{a_j}_j(t) = \{Y_{ij}(s;a_j), w_i(a_j) : s \leq t, i = 1, \ldots, n\}$$

which contains the counterfactual history of all units under treatment $a_j$, for $j = 1, 2$. We want to show that

$$M_j(t;a_j) = \int_0^t \left\{dN_j(s;a_j) - Y_j(s;a_j)d\Lambda_j^{a_j}(s)\right\}$$

is a martingale with respect to $\mathcal{F}^{a_j}_j(t)$. In fact,

$$\begin{aligned}
&E\{dM_j(t;a_j) \mid \mathcal{F}^{a_j}_j(t)\} \\
&= E\{dN_j(t;a_j) - Y_j(t;a_j)d\Lambda_j^{a_j}(t) \mid \mathcal{F}^{a_j}_j(t)\} \\
&= E\left[E\{dN_j(t;a_j) - Y_j(t;a_j)d\Lambda_j^{a_j}(t) \mid \mathcal{F}^{a_j}_j(t), X_1, \ldots, X_n\} \mid \mathcal{F}^{a_j}_j(t)\right] \\
&= E\left[E\left\{\sum_{i=1}^n w_i(a_j)\left\{dN_{ij}(t;a_j) - Y_{ij}(t;a_j)d\Lambda_j^{a_j}(t)\right\} \mid \mathcal{F}^{a_j}_j(t), X_1, \ldots, X_n\right\} \mid \mathcal{F}^{a_j}_j(t)\right] \\
&= E\left[\sum_{i=1}^n w_i(a_j)\left\{Y_{ij}(t;a_j)d\Lambda_j^{a_j}(t;X_i) - Y_{ij}(t;a_j)d\Lambda_j^{a_j}(t)\right\} \mid \mathcal{F}^{a_j}_j(t)\right]
\end{aligned}$$

$$
\begin{aligned}
&= \sum_{i=1}^{n} w_i(a_j)Y_{ij}(t;a_j)E\{d\Lambda_j^{a_j}(t;X_i) \mid \mathcal{F}_j^{a_j}(t)\} - \sum_{i=1}^{n} w_i(a_j)Y_{ij}(t;a_j)d\Lambda_j^{a_j}(t) \\
&= \sum_{i=1}^{n} w_i(a_j)Y_{ij}(t;a_j)\int_{\mathcal{X}} P\left(X_i = x \mid Y_{ij}(t;a_j), w_i(a_j)\right) d\Lambda_j^{a_j}(t;x)dx - \sum_{i=1}^{n} w_i(a_j)Y_{ij}(t;a_j)d\Lambda_j^{a_j}(t) \\
&= \sum_{i=1}^{n} w_i(a_j)Y_{ij}(t;a_j)\int_{\mathcal{X}} \frac{P\left(dN_{ij}(t) = 1 \mid X_i = x\right) P\left(X_i = x \mid Y_{ij}(t;a_j), w_i(a_j)\right)}{P\left(Y_{ij}(t;a_j) = 1 \mid X_i = x\right)} dx \\
&\qquad - \sum_{i=1}^{n} w_i(a_j)Y_{ij}(t;a_j)d\Lambda_j^{a_j}(t).
\end{aligned}
$$

Note that only when $Y_{ij}(t;a_j) = 1$ can the integration contribute a non-zero term to the summation, so we only need to care about

$$
P\left(X_i = x \mid Y_{ij}(t;a_j) = 1, w_i(a_j)\right).
$$

Also note that when $I(A_i = a_j) = 1$ and $X_i = x$, the weight

$$
w_i(a_j) = \frac{1}{P(A_i = a_j \mid X_i)}
$$

is a function of $X_i = x$, so

$$
\begin{aligned}
&P\left(X_i = x \mid Y_{ij}(t;a_j) = 1, w_i(a_j)\right) \\
&= \frac{P\left(Y_{ij}(t;a_j) = 1 \mid X_i = x, w_i(a_j)\right) P\left(X_i = x, w_i(a_j)\right)}{\int_{\mathcal{X}} P\left(Y_{ij}(t;a_j) = 1 \mid X_i = x, w_i(a_j)\right) P\left(X_i = x, w_i(a_j)\right) dx} \\
&= \frac{P\left(Y_{ij}(t;a_j) = 1 \mid X_i = x\right) P\left(X_i = x\right)}{\int_{\mathcal{X}} P\left(Y_{ij}(t;a_j) = 1 \mid X_i = x\right) P\left(X_i = x\right) dx} \\
&= \frac{P\left(Y_{ij}(t;a_j) = 1 \mid X_i = x\right) P\left(X_i = x\right)}{P\left(Y_{ij}(t;a_j) = 1\right)}.
\end{aligned}
$$

Therefore,

$$
\begin{aligned}
&\sum_{i=1}^{n} w_i(a_j)Y_{ij}(t;a_j)\int_{\mathcal{X}} \frac{P\left(dN_{ij}(t) = 1 \mid X_i = x\right) P\left(X_i = x \mid Y_{ij}(t;a_j), w_i(a_j)\right)}{P\left(Y_{ij}(t;a_j) = 1 \mid X_i = x\right)} dx \\
&\qquad - \sum_{i=1}^{n} w_i(a_j)Y_{ij}(t;a_j)d\Lambda_j^{a_j}(t) \\
&= \sum_{i=1}^{n} w_i(a_j)Y_{ij}(t;a_j)\int_{\mathcal{X}} \frac{P\left(dN_{ij}(t) = 1 \mid X_i = x\right) P\left(X_i = x\right)}{P\left(Y_{ij}(t;a_j) = 1\right)} dx - \sum_{i=1}^{n} w_i(a_j)Y_{ij}(t;a_j)d\Lambda_j^{a_j}(t) \\
&= \sum_{i=1}^{n} w_i(a_j)Y_{ij}(t;a_j)\frac{P(t \le T_i^{a_j} < t + dt, R_i^{a_j} \ge t, C_i^{a_j} \ge t)}{P(T_i^{a_j} \ge t, R_i^{a_j} \ge t, C_i^{a_j} \ge t)} - \sum_{i=1}^{n} w_i(a_j)Y_{ij}(t;a_j)d\Lambda_j^{a_j}(t) \\
&= \sum_{i=1}^{n} w_i(a_j)Y_{ij}(t;a_j)d\Lambda_j^{a_j}(t) - \sum_{i=1}^{n} w_i(a_j)Y_{ij}(t;a_j)d\Lambda_j^{a_j}(t) \\
&= 0.
\end{aligned}
$$

The variance $\mathrm{var}\{dM_j(t;a_j) \mid \mathcal{F}_j^{a_j}(t)\}$ can be derived as follows.

$$
\mathrm{var}\{dM_j(t;a_j) \mid \mathcal{F}_j^{a_j}(t)\}
$$

$$
\begin{aligned}
&= \operatorname{var}\left[\sum_{i=1}^{n} w_i(a_j)\{dN_{ij}(t;a_j) - Y_{ij}(t;a_j)d\Lambda_j^{a_j}(t)\} \mid \mathcal{F}_j^{a_j}(t)\right] \\
&= \sum_{i=1}^{n} w_i(a_j)^2 \operatorname{var}\{dN_{ij}(t;a_j) - Y_{ij}(t;a_j)d\Lambda_j^{a_j}(t) \mid \mathcal{F}_j^{a_j}(t)\} \\
&= \sum_{i=1}^{n} w_i(a_j)^2 \operatorname{var}\{dN_{ij}(t;a_j) \mid \mathcal{F}_j^{a_j}(t)\} \\
&= \sum_{i=1}^{n} w_i(a_j)^2 \Big( E\left[\operatorname{var}\{dN_{ij}(t;a_j) \mid \mathcal{F}_j^{a_j}(t), X_1, \ldots, X_n\} \mid \mathcal{F}_j^{a_j}(t)\right] \\
&\qquad\qquad + \operatorname{var}\left[E\{dN_{ij}(t;a_j) \mid \mathcal{F}_j^{a_j}(t), X_1, \ldots, X_n\} \mid \mathcal{F}_j^{a_j}(t)\right] \Big) \\
&= \sum_{i=1}^{n} w_i(a_j)^2 E[Y_{ij}(t;a_j)d\Lambda_j^{a_j}(t;X_i)\{1 - d\Lambda_j^{a_j}(t;X_i)\} \mid \mathcal{F}_j^{a_j}(t)] \\
&\qquad\qquad + \sum_{i=1}^{n} w_i(a_j)^2 \operatorname{var}\{Y_{ij}(t;a_j)d\Lambda_j^{a_j}(t;X_i) \mid \mathcal{F}_j^{a_j}(t)\} \\
&= \sum_{i=1}^{n} w_i(a_j)^2 E\{Y_{ij}(t;a_j)d\Lambda_j^{a_j}(t;X_i) \mid \mathcal{F}_j^{a_j}(t)\} \\
&\qquad\qquad + \sum_{i=1}^{n} w_i(a_j)^2 Y_{ij}(t;a_j) \operatorname{var}\{d\Lambda_j^{a_j}(t;X_i) \mid \mathcal{F}_j^{a_j}(t)\} \\
&= \sum_{i=1}^{n} w_i(a_j)^2 Y_{ij}(t;a_j)d\Lambda_j^{a_j}(t) + \sum_{i=1}^{n} w_i(a_j)^2 Y_{ij}(t;a_j)E[\{d\Lambda_j^{a_j}(t;X_i) - d\Lambda_j^{a_j}(t)\}^2 \mid \mathcal{F}_j^{a_j}(t)] \\
&= \sum_{i=1}^{n} w_i(a_j)^2 Y_{ij}(t;a_j)d\Lambda_j^{a_j}(t),
\end{aligned}
$$

because the square of a differentiation is zero. To simplify notations, let

$$
\begin{aligned}
Y_1^w(t;a_1) &= \sum_{i=1}^{n} w_i(a_j)^2 Y_{i1}(t;a_1) = \sum_{i=1}^{n} \frac{1}{P(A_i = a_1 \mid X_i)^2} I\{\widetilde{T}_i \geq t, \widetilde{R}_i \geq t, A_i = a_1\}, \\
Y_2^w(t;a_2) &= \sum_{i=1}^{n} w_i(a_j)^2 Y_{i2}(t;a_2) = \sum_{i=1}^{n} \frac{1}{P(A_i = a_2 \mid X_i)^2} I\{\widetilde{T}_i \geq t, \widetilde{R}_i \geq t, A_i = a_2\}.
\end{aligned}
$$

Since $N_3(t;r,a_3)$, $Y_3(t;r,a_3)$ and $M_3(t;r,a_3)$ rely on an additional parameter $r$, they may not be very useful because the at-risk set would have zero probability at almost every $r \in [0,\tau]$. Two assumptions can be made to simplify them. The first is Markov assumption, $d\Lambda_3^{a_3}(t;r) = d\Lambda_{3,\text{ma.}}^{a_3}(t)$, under which

$$
\begin{aligned}
d\Lambda_3^{a_3}(t;r) &= P(t \leq T^{a_3} < t + dt \mid T^{a_3} \geq t, R^{a_3} = r) \\
&= P(t \leq T^{a_3} < t + dt \mid T^{a_3} \geq t, R^{a_3} = r, C^{a_3} \geq t) \\
&= P(t \leq T^{a_3} < t + dt \mid T^{a_3} \geq t, R^{a_3} \leq T^{a_3}, C^{a_3} \geq t)
\end{aligned}
$$

because the expression should be irrelevant to $r$ given $t$. So we can let

$$
N_3(t;a_3) := \sum_{i=1}^{n} w_i(a_3) N_{i3}(t;a_3) := \sum_{i=1}^{n} w_i(a_3) I(T_i^{a_3} \leq t, R_i^{a_3} \leq t, C_i^{a_3} \geq t)
$$

$$
\begin{aligned}
&= \sum_{i=1}^{n} w_i(a_3) I(\widetilde{T}_i \le t, \delta_i^T \delta_i^R = 1),\\
Y_3(t; a_3) : &= \sum_{i=1}^{n} w_i(a_3) Y_{i3}(t; a_3) := \sum_{i=1}^{n} w_i(a_3) I(T_i^{a_3} \ge t, R_i^{a_3} \le t, C_i^{a_3} \ge t)\\
&= \sum_{i=1}^{n} w_i(a_3) I\{\widetilde{T}_i \ge t, \widetilde{R}_i \le t, \delta_i^R = 1\},\\
Y_3^w(t; a_3) : &= \sum_{i=1}^{n} w_i(a_3)^2 I\{\widetilde{T}_i \ge t, \widetilde{R}_i \le t, \delta_i^R = 1\},\\
M_3(t; a_3) : &= \int_0^t \left\{ dN_3(s; a_3) - Y_3(s; a_3) d\Lambda_{3,\text{ma.}}^{a_3}(s) \right\}.
\end{aligned}
$$

The second is the semi-Markov assumption $d\Lambda_3^{a_3}(t; r) = d\Lambda_{3,\text{sm.}}^{a_3}(t - r)$, under which

$$
\begin{aligned}
d\Lambda_3^{a_3}(t; r) &= P(t \le T^{a_3} < t + dt \mid T^{a_3} \ge t, R^{a_3} = r)\\
&= P(t \le T^{a_3} < t + dt \mid T^{a_3} \ge t, R^{a_3} = r, C^{a_3} \ge t)\\
&= P(u \le T^{a_3} - R^{a_3} < u + du \mid T^{a_3} - R^{a_3} \ge u, R^{a_3} = r, C^{a_3} \ge R^{a_3} + u)\\
&= P(u \le T^{a_3} - R^{a_3} < u + du \mid T^{a_3} - R^{a_3} \ge u, C^{a_3} - R^{a_3} \ge u)
\end{aligned}
$$

because the expression should be irrelevant to $r$ given $u = t - r$. So we can let

$$
\begin{aligned}
N_3(u; a_3) : &= \sum_{i=1}^{n} w_i(a_3) N_{i3}(u; a_3) := \sum_{i=1}^{n} w_i(a_3) I(T_i^{a_3} - R_i^{a_3} \le u, C_i^{a_3} - R_i^{a_3} \ge u)\\
&= \sum_{i=1}^{n} w_i(a_3) I\{\widetilde{T}_i - \widetilde{R}_i \le u, \delta_i^T \delta_i^R = 1\},\\
Y_3(u; a_3) : &= \sum_{i=1}^{n} w_i(a_3) Y_{i3}(u; a_3) := \sum_{i=1}^{n} w_i(a_3) I(T_i^{a_3} - R_i^{a_3} \ge u, C_i^{a_3} - R_i^{a_3} \ge u)\\
&= \sum_{i=1}^{n} w_i(a_3) I\{\widetilde{T}_i - \widetilde{R}_i \ge u, \delta_i^R = 1\},\\
Y_3^w(u; a_3) : &= \sum_{i=1}^{n} w_i(a_3)^2 I\{\widetilde{T}_i - \widetilde{R}_i \ge u, \delta_i^R = 1\},\\
M_3(u; a_3) : &= \int_0^u \left\{ dN_3(s; a_3) - Y_3(s; a_3) d\Lambda_{3,\text{sm.}}^{a_3}(s) \right\}.
\end{aligned}
$$

To ensure that $Y_3(u; a_3)$ is left-continuous, we may assume that the intermediate event happens just before the primary event if $R_i = T_i$. We can show that $M_3(t; a_3)$ is a martingale with respect to $\mathcal{F}_3^{a_3}(t) = \{Y_{i3}(s; a_3), w_i(a_3) : s \le t, i = 1, \ldots, n\}$ similar with the proof for $M_1(t; a_1)$ or $M_2(t; a_2)$.

## B.2 Theorem 2: Asymptotic convergence

We first show that

$$
\widehat{\Lambda}_j^{a_j}(t) = \int_0^t \frac{dN_j(s; a_j)}{Y_j(s; a_j)}
$$

is an unbiased estimator for $\Lambda_j^{a_j}(t)$, where $j = 1, 2, 3$(ma. or sm.). In fact,

$$\begin{aligned}
E\{\widehat{\Lambda}_j^{a_j}(t)\} &= E\left\{\int_0^t \frac{dN_j(s;a_j)}{Y_j(s;a_j)}\right\} \\
&= E\left[E\left\{\int_0^t \frac{dN_j(s;a_j)}{Y_j(s;a_j)} \mid \mathcal{F}_j^{a_j}(s)\right\}\right] \\
&= E\left[\int_0^t \frac{E\{dN_j(s;a_j) \mid \mathcal{F}_j^{a_j}(s)\}}{Y_j(s;a_j)}\right] \\
&= E\left\{\int_0^t \frac{Y_j(s;a_j)d\Lambda_j^{a_j}(s)}{Y_j(s;a_j)}\right\} \\
&= E\left\{\int_0^t d\Lambda_j^{a_j}(s)\right\} \\
&= \Lambda_j^{a_j}(t),
\end{aligned}$$

and

$$\begin{aligned}
\mathrm{var}\{\widehat{\Lambda}_j^{a_j}(t)\} &= \mathrm{var}\left\{\int_0^t \frac{dN_j(s;a_j)}{Y_j(s;a_j)}\right\} \\
&= \mathrm{var}\left\{\int_0^t \frac{dN_j(s;a_j)}{Y_j(s;a_j)} - \int_0^t \frac{Y_j(s;a_j)d\Lambda_j^{a_j}(s)}{Y_j(s;a_j)}\right\} \\
&= \mathrm{var}\left\{\int_0^t \frac{dM_j(s;a_j)}{Y_j(s;a_j)}\right\} \\
&= E\left[\int_0^t \frac{\mathrm{var}\{dN_j(s;a_j) \mid \mathcal{F}_j^{a_j}(s)\}}{Y_j(s;a_j)^2}\right] \\
&= E\left\{\int_0^t \frac{Y_j^w(s;a_j)d\Lambda_j^{a_j}(s)}{Y_j(s;a_j)^2}\right\}
\end{aligned}$$

since $Y_j(s;a_j)$ is a predictable process and $Y_j^w(s;a_j)d\Lambda_j^{a_j}(s)$ is the compensator of $dM_j(s;a_j)$ (see Lemma 1). As an analogue of the property of Nelson–Aalen estimators,

$$n^{1/2}\left[E\int_0^t \frac{\{Y_j^w(s;a_j)/n\}d\Lambda_j^{a_j}(s)}{\{Y_j(s;a_j)/n\}^2}\right]^{-1/2}\{\widehat{\Lambda}_j^{a_j}(t) - \Lambda_j^{a_j}(t)\} \xrightarrow{d} N(0,1),$$

or substituting the limit of the asymptotic variance,

$$n^{1/2}\{\widehat{\Lambda}_j^{a_j}(t) - \Lambda_j^{a_j}(t)\} \xrightarrow{d} N\left\{0,\ \int_0^t \frac{E\{Y_j^w(s;a_j)/n\}d\Lambda_j^{a_j}(s)}{E\{Y_j(s;a_j)/n\}^2}\right\}.$$

It is easy to see that

$$\widehat{\mathrm{var}}\{\widehat{\Lambda}_j^{a_j}(t)\} = \int_0^t \frac{Y_j^w(s;a_j)d\widehat{\Lambda}_j^{a_j}(s)}{Y_j(s;a_j)^2}$$

is an unbiased estimator for

$$\mathrm{var}\{\widehat{\Lambda}_j^{a_j}(t)\} = E\int_0^t \frac{Y_j^w(s;a_j)d\Lambda_j^{a_j}(s)}{Y_j(s;a_j)^2}.$$

Now we discuss $\widehat{F}_1^a(t)$, $\widehat{F}_2^a(t)$ and $\widehat{F}_3^a(t)$ respectively. First,

$$\begin{aligned}
&\widehat{F}_1^a(t) - F_1^a(t) \\
&= \int_0^t \exp\{-\widehat{\Lambda}_1^{a_1}(s) - \widehat{\Lambda}_2^{a_2}(s)\} d\widehat{\Lambda}_1^{a_1}(s) - \int_0^t \exp\{-\Lambda_1^{a_1}(s) - \Lambda_2^{a_2}(s)\} d\Lambda_1^{a_1}(s) \\
&= \int_0^t \exp\{-\Lambda_1^{a_1}(s) - \Lambda_2^{a_2}(s)\}\{1 + \Lambda_1^{a_1}(s) + \Lambda_2^{a_2}(s) - \widehat{\Lambda}_1^{a_1}(s) - \widehat{\Lambda}_2^{a_2}(s)\} \left\{ d\Lambda_1^{a_1}(s) + \frac{dM_1(s;a_1)}{Y_1(s;a_1)} \right\} \\
&\qquad - \int_0^t \exp\{-\Lambda_1^{a_1}(s) - \Lambda_2^{a_2}(s)\} d\Lambda_1^{a_1}(s) + o_p(n^{-1/2}) \\
&= \int_0^t \exp\{-\Lambda_1^{a_1}(s) - \Lambda_2^{a_2}(s)\}\{\Lambda_1^{a_1}(s) + \Lambda_2^{a_2}(s) - \widehat{\Lambda}_1^{a_1}(s) - \widehat{\Lambda}_2^{a_2}(s)\} \left\{ d\Lambda_1^{a_1}(s) + \frac{dM_1(s;a_1)}{Y_1(s;a_1)} \right\} \\
&\qquad + \int_0^t \exp\{-\Lambda_1^{a_1}(s) - \Lambda_2^{a_2}(s)\} \frac{dM_1(s;a_1)}{Y_1(s;a_1)} + o_p(n^{-1/2}) \\
&= -\int_0^t \exp\{-\Lambda_1^{a_1}(s) - \Lambda_2^{a_2}(s)\} \left\{ \int_0^s \frac{dM_1(u;a_1)}{Y_1(u;a_1)} + \int_0^s \frac{dM_2(u;a_2)}{Y_2(u;a_2)} \right\} \left\{ d\Lambda_1^{a_1}(s) + \frac{dM_1(s;a_1)}{Y_1(s;a_1)} \right\} \\
&\qquad + \int_0^t \exp\{-\Lambda_1^{a_1}(s) - \Lambda_2^{a_2}(s)\} \frac{dM_1(s;a_1)}{Y_1(s;a_1)} + o_p(n^{-1/2}) \\
&= -\int_0^t \exp\{-\Lambda_1^{a_1}(s) - \Lambda_2^{a_2}(s)\} \left\{ \int_0^s \frac{dM_1(u;a_1)}{Y_1(u;a_1)} + \int_0^s \frac{dM_2(u;a_2)}{Y_2(u;a_2)} \right\} d\Lambda_1^{a_1}(s) \\
&\qquad + \int_0^t \exp\{-\Lambda_1^{a_1}(s) - \Lambda_2^{a_2}(s)\} \frac{dM_1(s;a_1)}{Y_1(s;a_1)} + o_p(n^{-1/2}) \\
&= -\int_0^t \int_s^t \exp\{-\Lambda_1^{a_1}(u) - \Lambda_2^{a_2}(u)\} d\Lambda_1^{a_1}(u) \left\{ \frac{dM_1(u;a_1)}{Y_1(s;a_1)} + \frac{dM_2(s;a_2)}{Y_2(u;a_2)} \right\} \\
&\qquad + \int_0^t \exp\{-\Lambda_1^{a_1}(s) - \Lambda_2^{a_2}(s)\} \frac{dM_1(s;a_1)}{Y_1(s;a_1)} + o_p(n^{-1/2}) \\
&= \int_0^t \left[ \exp\{-\Lambda_1^{a_1}(s) - \Lambda_2^{a_2}(s)\} - \int_s^t \exp\{-\Lambda_1^{a_1}(u) - \Lambda_2^{a_2}(u)\} d\Lambda_1^{a_1}(u) \right] \frac{dM_1(s;a_1)}{Y_1(s;a_1)} \\
&\qquad - \int_0^t \left[ \int_s^t \exp\{-\Lambda_1^{a_1}(u) - \Lambda_2^{a_2}(u)\} d\Lambda_1^{a_1}(u) \right] \frac{dM_2(s;a_2)}{Y_2(s;a_2)} + o_p(n^{-1/2}).
\end{aligned}$$

Similarly,

$$\begin{aligned}
\widehat{F}_2^a(t) - F_2^a(t) = &\int_0^t \left[ \exp\{-\Lambda_1^{a_1}(s) - \Lambda_2^{a_2}(s)\} - \int_s^t \exp\{-\Lambda_1^{a_1}(u) - \Lambda_2^{a_2}(u)\} d\Lambda_2^{a_2}(u) \right] \frac{dM_2(s;a_1)}{Y_2(s;a_2)} \\
&- \int_0^t \left[ \int_s^t \exp\{-\Lambda_1^{a_1}(u) - \Lambda_2^{a_2}(u)\} d\Lambda_2^{a_2}(u) \right] \frac{dM_1(s;a_1)}{Y_1(s;a_1)} + o_p(n^{-1/2}).
\end{aligned}$$

Next we consider $\widehat{F}_2(t) - \widehat{F}_3(t)$,

$$\begin{aligned}
&\{\widehat{F}_2^a(t) - F_2^a(t)\} - \{\widehat{F}_3^a(t) - F_3^a(t)\} \\
&= \int_0^t \exp\{-\widehat{\Lambda}_1^{a_1}(s) - \widehat{\Lambda}_2^{a_2}(s) - \widehat{\Lambda}_3^{a_3}(t;s)\} d\widehat{\Lambda}_2^{a_2}(s) - \int_0^t \exp\{-\Lambda_1^{a_1}(s) - \Lambda_2^{a_2}(s) - \Lambda_3^{a_3}(t;s)\} d\Lambda_2^{a_2}(s) \\
&= \int_0^t \exp\{-\Lambda_1^{a_1}(s) - \Lambda_2^{a_2}(s) - \Lambda_3^{a_3}(t;s)\}\{1 + \Lambda_1^{a_1}(s) + \Lambda_2^{a_2}(s) + \Lambda_3^{a_3}(t;s) - \widehat{\Lambda}_1^{a_1}(s) - \widehat{\Lambda}_2^{a_2}(s) - \widehat{\Lambda}_3^{a_3}(t;s)\}
\end{aligned}$$

$$
\left\{d\Lambda_2^{a_2}(s) + \frac{dM_2(s;a_2)}{Y_2(s;a_2)}\right\} - \int_0^t \exp\{-\Lambda_1^{a_1}(s) - \Lambda_2^{a_2}(s) - \Lambda_3^{a_3}(t;s)\} d\Lambda_2^{a_2}(s) + o_p(n^{-1/2})
$$

$$
= \int_0^t \exp\{-\Lambda_1^{a_1}(s) - \Lambda_2^{a_2}(s) - \Lambda_3^{a_3}(t;s)\}\{\Lambda_1^{a_1}(s) + \Lambda_2^{a_2}(s) + \Lambda_3^{a_3}(t;s) - \widehat{\Lambda}_1^{a_1}(s) - \widehat{\Lambda}_2^{a_2}(s) - \widehat{\Lambda}_3^{a_3}(t;s)\}
$$

$$
\left\{d\Lambda_2^{a_2}(s) + \frac{dM_2(s;a_2)}{Y_2(s;a_2)}\right\} + \int_0^t \exp\{-\Lambda_1^{a_1}(s) - \Lambda_2^{a_2}(s) - \Lambda_3^{a_3}(t;s)\} \frac{dM_2(s;a_2)}{Y_2(s;a_2)} + o_p(n^{-1/2})
$$

$$
= -\int_0^t \exp\{-\Lambda_1^{a_1}(s) - \Lambda_2^{a_2}(s) - \Lambda_3^{a_3}(t;s)\} \left[\int_0^s \left\{\frac{dM_1(u;a_1)}{Y_1(u;a_1)} + \frac{dM_2(u;a_2)}{Y_2(u;a_2)}\right\} + \int_s^t \frac{dM_3(u;s,a_3)}{Y_3(u;s,a_3)}\right]
$$

$$
\left\{d\Lambda_2^{a_2}(s) + \frac{dM_2(s;a_2)}{Y_2(s;a_2)}\right\} + \int_0^t \exp\{-\Lambda_1^{a_1}(s) - \Lambda_2^{a_2}(s) - \Lambda_3^{a_3}(t;s)\} \frac{dM_2(s;a_2)}{Y_2(s;a_2)} + o_p(n^{-1/2})
$$

$$
= -\int_0^t \exp\{-\Lambda_1^{a_1}(s) - \Lambda_2^{a_2}(s) - \Lambda_3^{a_3}(t;s)\} \int_0^s \left\{\frac{dM_1(u;a_1)}{Y_1(u;a_1)} + \frac{dM_2(u;a_2)}{Y_2(u;a_2)}\right\} d\Lambda_2^{a_2}(s)
$$

$$
- \int_0^t \exp\{-\Lambda_1^{a_1}(s) - \Lambda_2^{a_2}(s) - \Lambda_3^{a_3}(t;s)\} \int_s^t \frac{dM_3(u;s,a_3)}{Y_3(u;s,a_3)} d\Lambda_2^{a_2}(s)
$$

$$
+ \int_0^t \exp\{-\Lambda_1^{a_1}(s) - \Lambda_2^{a_2}(s) - \Lambda_3^{a_3}(t;s)\} \frac{dM_2(s;a_2)}{Y_2(s;a_2)} + o_p(n^{-1/2})
$$

$$
= -\int_0^t \left[\int_s^t \exp\{-\Lambda_1^{a_1}(u) - \Lambda_2^{a_2}(u) - \Lambda_3^{a_3}(t;u)\} d\Lambda_2^{a_2}(u)\right] \frac{dM_1(s;a_1)}{Y_1(s;a_1)}
$$

$$
+ \int_0^t \left[\exp\{-\Lambda_1^{a_1}(s) - \Lambda_2^{a_2}(s) - \Lambda_3^{a_3}(t;s)\}\right.
$$

$$
\left. - \int_s^t \exp\{-\Lambda_1^{a_1}(u) - \Lambda_2^{a_2}(u) - \Lambda_3^{a_3}(t;u)\} d\Lambda_2^{a_2}(u)\right] \frac{dM_2(s;a_2)}{Y_2(s;a_2)}
$$

$$
- \int_0^t \exp\{-\Lambda_1^{a_1}(s) - \Lambda_2^{a_2}(s) - \Lambda_3^{a_3}(t;s)\} \int_s^t \frac{dM_3(u;s,a_3)}{Y_3(u;s,a_3)} d\Lambda_2^{a_2}(s) + o_p(n^{-1/2}).
$$

Therefore,

$$
\widehat{F}^a(t) - F^a(t)
$$

$$
= \{\widehat{F}_1^a(t) - F_1^a(t)\} + \{\widehat{F}_3^a(t) - F_3^a(t)\}
$$

$$
= \{\widehat{F}_1^a(t) - F_1^a(t)\} + \{\widehat{F}_2^a(t) - F_2^a(t)\} - [\{\widehat{F}_2^a(t) - F_2^a(t)\} - \{\widehat{F}_3^a(t) - F_3^a(t)\}]
$$

$$
= \int_0^t \left[\exp\{-\Lambda_1^{a_1}(s) - \Lambda_2^{a_2}(s)\} - \int_s^t \exp\{-\Lambda_1^{a_1}(u) - \Lambda_2^{a_2}(u)\}\{d\Lambda_1^{a_1}(u) + d\Lambda_1^{a_1}(u)\}\right.
$$

$$
\left. + \int_s^t \exp\{-\Lambda_1^{a_1}(u) - \Lambda_2^{a_2}(u) - \Lambda_3^{a_3}(t;u)\} d\Lambda_2^{a_2}(u)\right] \frac{dM_1(s;a_1)}{Y_1(s;a_1)}
$$

$$
+ \int_0^t \left[\exp\{-\Lambda_1^{a_1}(s) - \Lambda_2^{a_2}(s)\} - \int_s^t \exp\{-\Lambda_1^{a_1}(u) - \Lambda_2^{a_2}(u)\}\{d\Lambda_1^{a_1}(u) + d\Lambda_2^{a_2}(u)\}\right.
$$

$$
- \exp\{-\Lambda_1^{a_1}(s) - \Lambda_2^{a_2}(s) - \Lambda_3^{a_3}(t;s)\}
$$

$$
\left. + \int_s^t \exp\{-\Lambda_1^{a_1}(u) - \Lambda_2^{a_2}(u) - \Lambda_3^{a_3}(t;u)\} d\Lambda_2^{a_2}(u)\right] \frac{dM_2(s;a_2)}{Y_2(s;a_2)}
$$

$$
+ \int_0^t \exp\{-\Lambda_1^{a_1}(s) - \Lambda_2^{a_2}(s) - \Lambda_3^{a_3}(t;s)\} \int_s^t \frac{dM_3(u;s,a_3)}{Y_3(u;s,a_3)} d\Lambda_2^{a_2}(s) + o_p(n^{-1/2})
$$

$$
= \int_0^t \left[\exp\{-\Lambda_1^{a_1}(t) - \Lambda_2^{a_2}(t)\} + \int_s^t \exp\{-\Lambda_1^{a_1}(u) - \Lambda_2^{a_2}(u) - \Lambda_3^{a_3}(t;u)\} d\Lambda_2^{a_2}(u)\right] \frac{dM_1(s;a_1)}{Y_1(s;a_1)}
$$

$$+ \int_0^t \Big[ \exp\{-\Lambda_1^{a_1}(t) - \Lambda_2^{a_2}(t)\} - \exp\{-\Lambda_1^{a_1}(s) - \Lambda_2^{a_2}(s) - \Lambda_3^{a_3}(t;s)\}$$
$$+ \int_s^t \exp\{-\Lambda_1^{a_1}(u) - \Lambda_2^{a_2}(u) - \Lambda_3^{a_3}(t;u)\} d\Lambda_2^{a_2}(u) \Big] \frac{dM_2(s;a_2)}{Y_2(s;a_2)}$$
$$+ \int_0^t \exp\{-\Lambda_1^{a_1}(s) - \Lambda_2^{a_2}(s) - \Lambda_3^{a_3}(t;s)\} \int_s^t \frac{dM_3(u;s,a_3)}{Y_3(u;s,a_3)} d\Lambda_2^{a_2}(s) + o_p(n^{-1/2}).$$

Define

$$G_1^a(t) = \int_0^t \Big[ \exp\{-\Lambda_1^{a_1}(t) - \Lambda_2^{a_2}(t)\}$$
$$+ \int_s^t \exp\{-\Lambda_1^{a_1}(u) - \Lambda_2^{a_2}(u) - \Lambda_3^{a_3}(t;u)\} d\Lambda_2^{a_2}(u) \Big] \frac{dM_1(s;a_1)}{Y_1(s;a_1)},$$
$$G_2^a(t) = \int_0^t \Big[ \exp\{-\Lambda_1^{a_1}(t) - \Lambda_2^{a_2}(t)\} - \exp\{-\Lambda_1^{a_1}(s) - \Lambda_2^{a_2}(s) - \Lambda_3^{a_3}(t;s)\}$$
$$+ \int_s^t \exp\{-\Lambda_1^{a_1}(u) - \Lambda_2^{a_2}(u) - \Lambda_3^{a_3}(t;u)\} d\Lambda_2^{a_2}(u) \Big] \frac{dM_2(s;a_2)}{Y_2(s;a_2)},$$
$$G_3^a(t) = \int_0^t \exp\{-\Lambda_1^{a_1}(s) - \Lambda_2^{a_2}(s) - \Lambda_3^{a_3}(t;s)\} \int_s^t \frac{dM_3(u;s,a_3)}{Y_3(u;s,a_3)} d\Lambda_2^{a_2}(s).$$

In order that $G_1^a(t)$, $G_2^a(t)$ and $G_3^a(t)$ are independent processes, we only need that the jumps of $R_i$ and $T_i$ do not occur at identical times. If $R_i = T_i$, we treat this unit as that it jumps from State 0 to State 2 first at time $t$ and then immediately jump from State 2 to State 3 at time $t^+$. The variances of $G_1^a(t)$, $G_2^a(t)$ and $G_3^a(t)$ are at the constant scales. So

$$n^{1/2}\{\widehat{F}^a(t) - F^a(t)\} = n^{1/2}\{G_1^a(t) + G_2^a(t) + G_3^a(t)\} + o_p(1).$$

According to Rebolledo's theorem, the limiting distribution is Gaussian. In fact, the right-hand-side converges to a Gaussian process (Section 5.5 of Kalbfleisch and Prentice, 2011).

### B.3 Corollaries: Markov and semi-Markov

If $d\Lambda_3^{a_3}(t;r)$ is Markov, i.e., $d\Lambda_3^{a_3}(t;r) = d\Lambda_{3,\text{ma.}}^{a_3}(t)$,

$$G_1^a(t) = \int_0^t \Big[ \exp\{-\Lambda_1^{a_1}(t) - \Lambda_2^{a_2}(t)\}$$
$$+ \int_s^t \exp\{-\Lambda_1^{a_1}(u) - \Lambda_2^{a_2}(u) - \Lambda_3^{a_3}(t) + \Lambda_3^{a_3}(u)\} d\Lambda_2^{a_2}(u) \Big] \frac{dM_1(s;a_1)}{Y_1(s;a_1)}$$
$$= \int_0^t \Big[ \exp\{-\Lambda_1^{a_1}(t) - \Lambda_2^{a_2}(t)\}$$
$$- \exp\{\Lambda_3^{a_3}(s) - \Lambda_3^{a_3}(t)\} \int_0^s \exp\{-\Lambda_1^{a_1}(u) - \Lambda_2^{a_2}(u) - \Lambda_3^{a_3}(s) + \Lambda_3^{a_3}(u)\} d\Lambda_2^{a_2}(u)$$
$$+ \int_0^t \exp\{-\Lambda_1^{a_1}(u) - \Lambda_2^{a_2}(u) - \Lambda_3^{a_3}(t) + \Lambda_3^{a_3}(u)\} d\Lambda_2^{a_2}(u) \Big] \frac{dM_1(s;a_1)}{Y_1(s;a_1)}$$
$$= \int_0^t \Big[ 1 - F_1^a(t) - F_3^a(t) - \{F_2^a(s) - F_3^a(s)\} \exp\{\Lambda_3^{a_3}(s) - \Lambda_3^{a_3}(t)\} \Big] \frac{dM_1(s;a_1)}{Y_1(s;a_1)},$$

$$
\begin{aligned}
G_2^a(t) &= \int_0^t \Bigg[ \exp\{-\Lambda_1^{a_1}(t) - \Lambda_2^{a_2}(t)\} - \exp\{-\Lambda_1^{a_1}(s) - \Lambda_2^{a_2}(s) - \Lambda_3^{a_3}(t) + \Lambda_3^{a_3}(s)\} \\
&\quad + \int_s^t \exp\{-\Lambda_1^{a_1}(u) - \Lambda_2^{a_2}(u) - \Lambda_3^{a_3}(t) + \Lambda_3^{a_3}(u)\} d\Lambda_2^{a_2}(u) \Bigg] \frac{dM_2(s;a_2)}{Y_2(s;a_2)} \\
&= \int_0^t \Bigg[ 1 - F_1^a(t) - F_2^a(t) - \{1 - F_1^a(s) - F_2^a(s)\} \exp\{\Lambda_3^{a_3}(s) - \Lambda_3^{a_3}(t)\} \\
&\quad - \exp\{\Lambda_3^{a_3}(s) - \Lambda_3^{a_3}(t)\} \int_0^s \exp\{-\Lambda_1^{a_1}(u) - \Lambda_2^{a_2}(u) - \Lambda_3^{a_3}(s) + \Lambda_3^{a_3}(u)\} d\Lambda_2^{a_2}(u) \\
&\quad + \int_0^t \exp\{-\Lambda_1^{a_1}(u) - \Lambda_2^{a_2}(u) - \Lambda_3^{a_3}(t) + \Lambda_3^{a_3}(u)\} d\Lambda_2^{a_2}(u) \Bigg] \frac{dM_2(s;a_2)}{Y_2(s;a_2)} \\
&= \int_0^t \Bigg[ 1 - F_1^a(t) - F_3^a(t) - \{1 - F_1^a(s) - F_2^a(s)\} \exp\{\Lambda_3^{a_3}(s) - \Lambda_3^{a_3}(t)\} \\
&\quad - \{F_2^a(s) - F_3^a(s)\} \exp\{\Lambda_3^{a_3}(s) - \Lambda_3^{a_3}(t)\} d\Lambda_2^{a_2}(u) \Bigg] \frac{dM_2(s;a_2)}{Y_2(s;a_2)} \\
&= \int_0^t \Bigg[ 1 - F_1^a(t) - F_3^a(t) - \{1 - F_1^a(s) - F_3^a(s)\} \exp\{\Lambda_3^{a_3}(s) - \Lambda_3^{a_3}(t)\} \Bigg] \frac{dM_2(s;a_2)}{Y_2(s;a_2)}, \\
G_3^a(t) &= \int_0^t \exp\{-\Lambda_1^{a_1}(s) - \Lambda_2^{a_2}(s) - \Lambda_3^{a_3}(t) + \Lambda_3^{a_3}(s)\} \int_s^t \frac{dM_3(u;a_3)}{Y_3(u;a_3)} d\Lambda_2^{a_2}(s) \\
&= \int_0^t \Bigg[ \int_0^s \exp\{-\Lambda_1^{a_1}(u) - \Lambda_2^{a_2}(u) - \Lambda_3^{a_3}(t) + \Lambda_3^{a_3}(u)\} d\Lambda_2^{a_2}(u) \Bigg] \frac{dM_3(s;a_3)}{Y_3(s;a_3)} \\
&= \int_0^t \Bigg[ \int_0^s \exp\{-\Lambda_1^{a_1}(u) - \Lambda_2^{a_2}(u) - \Lambda_3^{a_3}(s) + \Lambda_3^{a_3}(u)\} d\Lambda_2^{a_2}(u) \\
&\quad \exp\{\Lambda_3^{a_3}(s) - \Lambda_3^{a_3}(t)\} \Bigg] \frac{dM_3(s;a_3)}{Y_3(s;a_3)} \\
&= \int_0^t \{F_2^a(s) - F_3^a(s)\} \exp\{\Lambda_3^{a_3}(s) - \Lambda_3^{a_3}(t)\} \frac{dM_3(s;a_3)}{Y_3(s;a_3)}.
\end{aligned}
$$

Note that $G_1^a(t)$, $G_2^a(t)$ and $G_3^a(t)$ are all compounds of predictable processes and martingales, so

$$
\begin{aligned}
\mathrm{var}\{G_1^a(t)\} &= E \int_0^t [1 - F_1^a(t) - F_3^a(t) - \{F_2^a(s) - F_3^a(s)\} \exp\{\Lambda_3^{a_3}(s) - \Lambda_3^{a_3}(t)\}]^2 \frac{Y_1^w(s;a_1)}{Y_1(s;a_1)^2} d\Lambda_1^{a_1}(s), \\
\mathrm{var}\{G_2^a(t)\} &= E \int_0^t [1 - F_1^a(t) - F_3^a(t) - \{1 - F_1^a(s) - F_3^a(s)\} \exp\{\Lambda_3^{a_3}(s) - \Lambda_3^{a_3}(t)\}]^2 \frac{Y_2^w(s;a_2)}{Y_2(s;a_2)^2} d\Lambda_2^{a_2}(s), \\
\mathrm{var}\{G_3^a(t)\} &= E \int_0^t [\{F_2^a(s) - F_3^a(s)\} \exp\{\Lambda_3^{a_3}(s) - \Lambda_3^{a_3}(t)\}]^2 \frac{Y_3^w(s;a_3)}{Y_3(s;a_3)^2} d\Lambda_3^{a_3}(s).
\end{aligned}
$$

Recall that $G_1^a(t)$, $G_2^a(t)$ and $G_3^a(t)$ are independent, finally

$$
n^{1/2}\{\widehat{F}^a(t) - F^a(t)\} \xrightarrow{d} N \left\{ 0,\ \lim_{n\to\infty} n \sum_{j=1}^{3} \mathrm{var}\{G_j^a(t)\} \right\}.
$$

By noting that $Y_1(t;a)/n = Y_2(t;a) \to P(T^a \wedge R^a \wedge C^a \geq t, A = a)$ and $Y_3(t;a)/n \to P(T^a \wedge C^a \geq t, R^a < t, A = a)$ uniformly in $[0, \tau]$, we have Corollary 1.

If $d\Lambda_3^{a_3}(t;r)$ is semi-Markov, i.e., $d\Lambda_3^{a_3}(t;r) = d\Lambda_{3,\mathrm{sm.}}^{a_3}(t-r)$,

$$
G_1^a(t) = \int_0^t \left[ \exp\{-\Lambda_1^{a_1}(t) - \Lambda_2^{a_2}(t)\} + \int_s^t \exp\{-\Lambda_1^{a_1}(u) - \Lambda_2^{a_2}(u) - \Lambda_3^{a_3}(t-u)\} d\Lambda_2^{a_2}(u) \right] \frac{dM_1(s;a_1)}{Y_1(s;a_1)}
$$

$$= \int_0^t \left[1 - F_1^a(t) - F_2^a(t) + \int_s^t \exp\{-\Lambda_3^{a_3}(t-u)\} dF_2^a(u)\right] \frac{dM_1(s;a_1)}{Y_1(s;a_1)},$$

$$G_2^a(t) = \int_0^t \left[\exp\{-\Lambda_1^{a_1}(t) - \Lambda_2^{a_2}(t)\} - \exp\{-\Lambda_1^{a_1}(s) - \Lambda_2^{a_2}(s) - \Lambda_3^{a_3}(t-s)\}\right.$$
$$\left. + \int_s^t \exp\{-\Lambda_1^{a_1}(u) - \Lambda_2^{a_2}(u) - \Lambda_3^{a_3}(t-u)\} d\Lambda_2^{a_2}(u)\right] \frac{dM_2(s;a_2)}{Y_2(s;a_2)}$$
$$= \int_0^t \left[1 - F_1^a(t) - F_2^a(t) - \{1 - F_1^a(s) - F_2^a(s)\} \exp\{-\Lambda_3^{a_3}(t-s)\}\right.$$
$$\left. + \int_s^t \exp\{-\Lambda_3^{a_3}(t-u)\} dF_2^a(u)\right] \frac{dM_2(s;a_2)}{Y_2(s;a_2)}$$
$$= \int_0^t \left[\{1 - F_1^a(u) - F_2^a(u)\} \exp\{-\Lambda_3^{a_3}(t-u)\}\Big|_s^t + \int_s^t \exp\{-\Lambda_3^{a_3}(t-u)\} dF_2^a(u)\right] \frac{dM_2(s;a_2)}{Y_2(s;a_2)},$$

$$G_3^a(t) = \int_0^t \exp\{-\Lambda_1^{a_1}(s) - \Lambda_2^{a_2}(s) - \Lambda_3^{a_3}(t-s)\} \int_s^t \frac{dM_3(u-s;a_3)}{Y_3(u-s;a_3)} d\Lambda_2^{a_2}(s)$$
$$= \int_0^t \exp\{-\Lambda_1^{a_1}(s) - \Lambda_2^{a_2}(s) - \Lambda_3^{a_3}(t-s)\} \int_0^{t-s} \frac{dM_3(u;a_3)}{Y_3(u;a_3)} d\Lambda_2^{a_2}(s)$$
$$= \int_0^t \left[\int_0^{t-s} \exp\{-\Lambda_1^{a_1}(u) - \Lambda_2^{a_2}(u) - \Lambda_3^{a_3}(t-u)\} d\Lambda_2^{a_2}(u)\right] \frac{dM_3(u;a_3)}{Y_3(u;a_3)}$$
$$= \int_0^t \left[\int_0^{t-s} \exp\{-\Lambda_3^{a_3}(t-u)\} dF_2^a(u)\right] \frac{dM_3(u;a_3)}{Y_3(u;a_3)}.$$

Note that $G_1^a(t)$, $G_2^a(t)$ and $G_3^a(t)$ are all compounds of predictable processes and martingales, so

$$\text{var}\{G_1^a(t)\} = E \int_0^t \left[1 - F_1^a(t) - F_2^a(t) + \int_s^t \exp\{-\Lambda_3^{a_3}(t-u)\} dF_2^a(u)\right]^2 \frac{Y_1^w(s;a_1)}{Y_1(s;a_1)^2} d\Lambda_1^{a_1}(s),$$
$$\text{var}\{G_2^a(t)\} = E \int_0^t \left[\{1 - F_1^a(u) - F_2^a(u)\} \exp\{-\Lambda_3^{a_3}(t-u)\}\Big|_s^t\right.$$
$$\left. + \int_s^t \exp\{-\Lambda_3^{a_3}(t-u)\} dF_2^a(u)\right]^2 \frac{Y_2^w(s;a_2)}{Y_2(s;a_2)^2} d\Lambda_2^{a_2}(s),$$
$$\text{var}\{G_3^a(t)\} = E \int_0^t \left[\int_0^{t-s} \exp\{-\Lambda_3^{a_3}(t-u)\} dF_2^a(u)\right]^2 \frac{Y_3^w(s;a_3)}{Y_3(s;a_3)^2} d\Lambda_3^{a_3}(s).$$

Recall that $G_1^a(t)$, $G_2^a(t)$ and $G_3^a(t)$ are independent, finally

$$n^{1/2}\{\widehat{F}^a(t) - F^a(t)\} \xrightarrow{d} N\left\{0,\ \lim_{n\to\infty} n \sum_{j=1}^3 \text{var}\{G_j^a(t)\}\right\}.$$

The limiting variance of $G_j^a(t)$ can be calculated by applying the law of large numbers to $Y_j(s;a_j)$ and $Y_j^w(s;a_j)$. By noting that $Y_1(t;a)/n = Y_2(t;a)/n \to P(T^a \wedge R^a \wedge C^a \geq t, A = a)$ and $Y_3(t;a)/n \to P(T^a \wedge C^a \geq t, R^a < t, A = a)$ uniformly in $[0, \tau]$, we have Corollary 2.

# C Proof of Theorem 3 (Uniform consistency)

As illustrated in Section B.2, we have

$$\widehat{F}^a(t) - F^a(t) = G_1^a(t) + G_2^a(t) + G_3^a(t) + R^a(t),$$

where $\sup_{t\in(0,\tau]} R^a(t) = o_p(n^{-1/2})$.

Let $H_1(t,s) = \left[\exp\{-\Lambda_1^{a_1}(t) - \Lambda_2^{a_2}(t)\} + \int_s^t \exp\{-\Lambda_1^{a_1}(u) - \Lambda_2^{a_2}(u) - \Lambda_3^{a_3}(t;u)\} d\Lambda_2^{a_2}(u)\right]$. Using Cauchy inequality, we have

$$\}Y_1^w(s;a_1)\}^2 = \left(\sum_i w_i^2 Y_{i1}\right)^2 \leq \sum_i w_i^2 \sum_i (w_i Y_{i1})^2 = \sum_i w_i^2 Y_1^w(s;a_1),$$

which leads to

$$Y_1^w(s;a_1) \leq \sum_i w_i^2 \leq n/c^2. \tag{1}$$

By the inequality of Lenglart, for positive $\eta$ and $\delta$, we have

$$\begin{aligned}
P\left[\sup_{t\in[0,\tau]} |G_1^a(t)| > \sqrt{\eta}\right] &\leq \frac{\delta}{\eta} + P\left[\int_0^\tau \frac{H_1^2(\tau,s)}{Y_1^2(s;a_1)} d\left\langle M_1\right\rangle(s;a_1) > \delta\right] \\
&\leq \frac{\delta}{\eta} + P\left[\int_0^\tau \frac{H_1^2(\tau,s)}{Y_1^2(s;a_1)} Y_1^w(s;a_1) d\Lambda_1^{a_1}(s) > \delta\right] \\
&\leq \frac{\delta}{\eta} + P\left[\int_0^\tau \frac{\left(1+\int_s^\tau d\Lambda_2^{a_2}(u)\right)^2}{Y_1^2(s;a_1)} Y_1^w(s;a_1) d\Lambda_1^{a_1}(s) > \delta\right] \\
&\leq \frac{\delta}{\eta} + P\left[\int_0^\tau \frac{n\left(1+\Lambda_2^{a_2}(\tau)\right)^2}{c^2 Y_1^2(s;a_1)} d\Lambda_1^{a_1}(s) > \delta\right] \\
&\leq \frac{\delta}{\eta} + P\left[\frac{n\left(1+\Lambda_2^{a_2}(\tau)\right)^2}{c^2 Y_1^2(\tau;a_1)} \Lambda_1^{a_1}(\tau) > \delta\right] \\
&\leq \frac{\delta}{\eta} + P\left[Y_1^2(\tau;a_1) < \frac{n\left(1+\Lambda_2^{a_2}(\tau)\right)^2 \Lambda_1^{a_1}(\tau)}{c^2\delta}\right].
\end{aligned}$$

The third inequality is due to $\Lambda_j^{a_j}(u) \geq 0$ for $j = 1,2,3$, the fourth inequality is due to equation (1), $Y_1(t;a_1)$ is non-increase leads to the fifth inequality.

Similarly, we can prove

$$P\left[\sup_{t\in[0,\tau]} |G_2^a(t)| > \sqrt{\eta}\right] \leq \frac{\delta}{\eta} + P\left[Y_2^2(\tau;a_2) < \frac{n\left(1+\Lambda_2^{a_2}(\tau)\right)^2 \Lambda_2^{a_2}(\tau)}{c^2\delta}\right].$$

Since

$$d\Lambda_3^{a_3}(t;r) = (1-\kappa) d\Lambda_{3,\text{ma.}}^{a_3}(t) + \kappa d\Lambda_{3,\text{sm.}}^{a_3}(t-r)$$

and proof in section B.3, we have

$$\begin{aligned}
G_3^a(t) = (1-\kappa) &\int_0^t \{F_2^a(s) - F_3^a(s)\} \exp\{\Lambda_{3,\text{ma.}}^{a_3}(s) - \Lambda_{3,\text{ma.}}^{a_3}(t)\} \frac{dM_{3,\text{ma.}}(s;a_3)}{Y_{3,\text{ma.}}(s;a_3)} \\
&+ \kappa \int_0^t \left[\int_0^{t-s} \exp\{-\Lambda_{3,\text{sm.}}^{a_3}(t-u)\} dF_2^a(u)\right] \frac{dM_{3,\text{sm.}}(s;a_3)}{Y_{3,\text{sm.}}(s;a_3)} \\
&:= (1-\kappa) G_{3,\text{ma.}}^a + \kappa G_{3,\text{sm.}}^a,
\end{aligned}$$

where

$$dM_{3,\text{ma.}}(s;a_3) = dN_3(s;a_3) - Y_{3,\text{ma.}}(s;a_3)d\Lambda_{3,\text{ma.}}(s),$$
$$dM_{3,\text{sm.}}(s;a_3) = dN_3(s;a_3) - Y_{3,\text{sm.}}(s;a_3)d\Lambda_{3,\text{sm.}}(s).$$

Similar to the proof of $G_1^a(t)$, we can prove

$$P\left[\sup_{t\in[0,\tau]} |G^a_{3,\text{ma.}}(t)| > \sqrt{\eta}\right] \leq \frac{\delta}{\eta} + P\left[Y_3^2(\tau;a_3) < \frac{n\Lambda^{a_3}_{3,\text{ma.}}(\tau)}{c^2\delta}\right]$$

and

$$P\left[\sup_{t\in[0,\tau]} |G^a_{3,\text{sm.}}(t)| > \sqrt{\eta}\right] \leq \frac{\delta}{\eta} + P\left[Y_3^2(\tau;a_3) < \frac{n\Lambda^{a_3}_{3,\text{sm.}}(\tau)}{c^2\delta}\right].$$

Therefore, we have

$$\begin{aligned}
&P\left[\sup_{t\in[0,\tau]} |\widehat{F}^a(t) - F^a(t)| > \sqrt{\eta}\right]\\
&\leq P\left[\sup_{t\in[0,\tau]} |G^a_1(t)| > \frac{\sqrt{\eta}}{5}\right] + P\left[\sup_{t\in[0,\tau]} |G^a_2(t)| > \frac{\sqrt{\eta}}{5}\right] + P\left[\sup_{t\in[0,\tau]} |G^a_{3,\text{ma.}}(t)| > \frac{\sqrt{\eta}}{5}\right]\\
&\quad + P\left[\sup_{t\in[0,\tau]} |G^a_{3,\text{sm.}}(t)| > \frac{\sqrt{\eta}}{5}\right] + P\left[\sup_{t\in[0,\tau]} |R^a(t)| > \frac{\sqrt{\eta}}{5}\right]\\
&\leq \frac{100\delta}{\eta} + P\left[Y_1^2(\tau;a_1) < \frac{n\left(1+\Lambda_2^{a_2}(\tau)\right)^2\Lambda_1^{a_1}(\tau)}{c^2\delta}\right] + P\left[Y_2^2(\tau;a_2) < \frac{n\left(1+\Lambda_2^{a_2}(\tau)\right)^2\Lambda_2^{a_2}(\tau)}{c^2\delta}\right]\\
&\quad + P\left[Y_3^2(\tau;a_3) < \frac{n\Lambda^{a_3}_{3,\text{ma.}}(\tau)}{c^2\delta}\right] + P\left[Y_3^2(\tau;a_3) < \frac{n\Lambda^{a_3}_{3,\text{sm.}}(\tau)}{c^2\delta}\right] + P\left[\sup_{t\in[0,\tau]} |R^a(t)| > \frac{\sqrt{\eta}}{5}\right]
\end{aligned}$$

On the other hand, $Y_j(\tau;a_j) \geq Cn^{1/2}$ for $j = 1,2,3$(ma., sm.) in probability as $n \to \infty$. As $\delta$ and $\eta$ are arbitrarily chosen, it is deduced that

$$P\left[\sup_{t\in[0,\tau]} |\widehat{F}^a(t) - F^a(t)| > \sqrt{\eta}\right] \to 0,$$

as $n \to \infty$. Therefore,

$$\sup_{t\in[0,\tau]} \left|\widehat{F}^a(t) - F^a(t)\right| \to 0$$

in probability.

# D Hypothesis testing for separable effects

## D.1 Hypothesis tests and test statistics

To detect on which pathways treatment effects exist, we shall conduct hypothesis tests on separable pathway effects $\text{SPE}_{0\to1}$, $\text{SPE}_{0\to2}$ and $\text{SPE}_{2\to3}$. We consider testing three potential hazards here:

$$H_0^j : d\Lambda_j^1(t) = d\Lambda_j^0(t), \forall t \in [0,\tau] \;\text{ v.s. }\; H_1^j : d\Lambda_j^1(t) \neq d\Lambda_j^0(t), \exists t \in [0,\tau], j = 1,2,3.$$

When the null hypothesis holds, the corresponding separable pathway effect is zero. But there is an exception for the inverse: $\text{SPE}_{0\to 2}(t;a_1,a_3)=0$ if either $H_0^2$ holds or $d\Lambda_1^{a_1}(t)=d\Lambda_3^{a_3}(t;s)$ (Huang, 2022). Define the weighted logrank statistics with a left-continuous weight $W(t)$ as

$$U_j=\int_0^\tau W(t)\frac{Y_j(t;1)dN_j(t;0)-Y_j(t;0)dN_j(t;1)}{Y_j(t;1)+Y_j(t;0)},\ j=1,2,3.$$

Test statistics can be constructed based on the following theorem.

**Theorem S1.** *Under the null hypothesis $H_0^j$, we have $n^{-1/2}U_j\xrightarrow{d}N(0,\sigma_j^2)$, where*

$$\sigma_j^2=\lim_{n\to\infty}E\left\{\int_0^\tau W(t)^2\frac{Y_j(t;1)^2Y_j^w(t;0)+Y_j(t;0)Y_j^w(t;1)}{n\{Y_j(t;1)+Y_j(t;0)\}^2}d\Lambda_j^{a_j}(t)\right\},\ j=1,2,3.$$

It is equivalent to express $\sigma_j^2$ by taking expectation with respect to $Y_j(t;a)$ and $Y_j^w(t;a)$ separately. The variances $\sigma_j^2$ can be asymptotically unbiasedly estimated by replacing $d\Lambda_j^{a_j}(\cdot)$ with its estimator in the expectations, denoted by $\widehat{\sigma}_j^2$. An asymptotic two-sided level $\alpha$ test for $H_0^j$ should reject the null hypothesis if $n^{-1/2}|U_j|/\widehat{\sigma}_j$ is larger than the $\alpha/2$ upper quantile of the standard normal distribution. These three tests can be combined by multiple testing techniques to yield joint tests.

## D.2 Proof of asymptotic properties of test statistics

For $j=1,2,3$(ma. or sm.), if $d\Lambda_j^1(t)=d\Lambda_j^0(t)$,

$$\begin{aligned}
E(U_j)&=E\left\{\int_0^\tau W(t)\frac{Y_j(t;1)dN_j(t;0)-Y_j(t;0)dN_j(t;1)}{Y_j(t;1)+Y_j(t;0)}\right\}\\
&=E\left[E\left\{\int_0^\tau W(t)\frac{Y_j(t;1)dN_j(t;0)-Y_j(t;0)dN_j(t;1)}{Y_j(t;1)+Y_j(t;0)}\mid \mathcal{F}_j^1(t),\mathcal{F}_j^0(t)\right\}\right]\\
&=E\left[\int_0^\tau W(t)\frac{Y_j(t;1)E\{dN_j(t;0)\mid\mathcal{F}_j^0(t)\}-Y_j(t;0)E\{dN_j(t;1)\mid\mathcal{F}_j^1(t)\}}{Y_j(t;1)+Y_j(t;0)}\right]\\
&=E\left\{\int_0^\tau W(t)\frac{Y_j(t;1)Y_j(t;0)d\Lambda_j^0(t)-Y_j(t;0)Y_j(t;1)d\Lambda_j^1(t)}{Y_j(t;1)+Y_j(t;0)}\right\}\\
&=0,
\end{aligned}$$

$$\begin{aligned}
\text{var}(U_j)&=\text{var}\left\{\int_0^\tau W(t)\frac{Y_j(t;1)dN_j(t;0)-Y_j(t;0)dN_j(t;1)}{Y_j(t;1)+Y_j(t;0)}\right\}\\
&=E\left[\text{var}\left\{\int_0^\tau W(t)\frac{Y_j(t;1)dN_j(t;0)-Y_j(t;0)dN_j(t;1)}{Y_j(t;1)+Y_j(t;0)}\mid \mathcal{F}_j^1(t),\mathcal{F}_j^0(t)\right\}\right]\\
&=E\left[\int_0^\tau W(t)^2\frac{Y_j(t;1)^2\,\text{var}\{dN_j(t;0)\mid\mathcal{F}_j^0(t)\}+Y_j(t;0)^2\,\text{var}\{dN_j(t;1)\mid\mathcal{F}_j^1(t)\}}{\{Y_j(t;1)+Y_j(t;0)\}^2}\mid \mathcal{F}_j^1(t),\mathcal{F}_j^0(t)\right]\\
&=E\left[\int_0^\tau W(t)^2\frac{Y_j(t;1)^2Y_j^w(t;0)d\Lambda_j^0(t)-Y_j(t;0)^2Y_j^w(t;1)d\Lambda_j^1(t)}{\{Y_j(t;1)+Y_j(t;0)\}^2}\right].
\end{aligned}$$

In most cases, we simply take $W(t)=1$. The order of $\text{var}(U_j)$ is $O(n)$. Let $\sigma_j^2=\lim_{n\to\infty}\text{var}(U_j)/n$, then

$$n^{-1/2}U_j\xrightarrow{d}N\left(0,\sigma_j^2\right).$$

An alternative strategy to test the hypotheses are using permutation tests that randomly permute treatment assignments $\{A_i : i = 1, \dots, n\}$. If the null hypothesis holds, then the statistics $U_j^{(b)}$ under the $b$th permutation should follow the same distribution and also have zero expectation. By comparing the realized statistic $U_j$ with the empirical distribution of $\{U_j^{(b)} : b = 1, \dots, B\}$, we can calculate the $p$-value of the permutation test. However, this strategy is time demanding, so we recommend logrank tests.

# E Efficient influence function in the general case

(Martinussen and Stensrud, 2023) has shown that the efficient influence function of $\Lambda_j^{a_j}(t; x)$ is given by $(j = 1, 2)$

$$\mathrm{EIF}\{\Lambda_j^{a_j}(t; x)\} = \frac{I(A = a_j)}{p(x)P(A = a_j \mid X = x)} \int_0^t \frac{dM_j(s; a_j, x)}{P(\widetilde{T} \wedge \widetilde{R} \geq s \mid A = a_j, X = x)}.$$

Similarly, by taking care to the at-risk set of the indirect outcome event, the efficient influence function of $\Lambda_3^{a_3}(t; r, x)$ is

$$\mathrm{EIF}\{\Lambda_3^{a_3}(t; r, x)\} = \frac{I(A = a_3)}{p(x)P(A = a_3 \mid X = x)} \int_0^t \frac{dM_3(s; r, a_3, x)}{P(\mathcal{H}(t, r) \mid A = a_3, X = x)}.$$

It is trivial that the efficient influence of $dP(x)$ is

$$\mathrm{EIF}\{dP(x)\} = I(X = x)dx - dP(x).$$

Let $dP_j(t; \mathcal{F}(t)) = \exp\{-\Lambda_j(t; \mathcal{F}(t))\}d\Lambda_j^{a_j}(t; \mathcal{F}(t))$ be the conditional density of transiting to State $j$ given the history $\mathcal{F}(t)$ including covariates. By the functional delta method, the efficient influence function of

$$F_1^a(t) = \int_{\mathcal{X}} \int_0^t dP_1(s; a_1, x)dP(x)$$

is

$$\begin{aligned}\varphi_1^a(t) = \int_{\mathcal{X}} \int_0^t dP_1(s; a_1, x) \bigg[ &\frac{\mathrm{EIF}\{d\Lambda_1^{a_1}(s; x)\}}{d\Lambda_1^{a_1}(s; x)} dP(x) \\ &- \sum_{j \in \{1,2\}} \mathrm{EIF}\{\Lambda_j^{a_j}(s; x)\}dP(x) + \mathrm{EIF}\{dP(x)\} \bigg].\end{aligned}$$

The efficient influence function of

$$F_3^a(t) = \int_{\mathcal{X}} \int_0^t \int_0^s dP_2(r; a_2, x)dP_3(s; r, a_3, x)dP(x)$$

is

$$\begin{aligned}\varphi_3^a(t) = \int_{\mathcal{X}} \int_0^t \int_0^s &dP_2(r; a_2, x)dP_3(s; r, a_3, x) \\ &\cdot \bigg[ \frac{\mathrm{EIF}\{d\Lambda_2^{a_2}(r; x)\}}{d\Lambda_2^{a_2}(r; x)} dP(x) - \sum_{j \in \{1,2\}} \mathrm{EIF}\{\Lambda_j^{a_j}(s; x)\}dP(x)\end{aligned}$$

$$+\frac{\mathrm{EIF}\{d\Lambda_3^{a_3}(s;r,x)\}}{d\Lambda_3^{a_3}(s;r,x)}dP(x)-\mathrm{EIF}\{\Lambda_3^{a_3}(s;r,x)\}dP(x)$$
$$\left.+\,\mathrm{EIF}\{dP(x)\}\right].$$

So the efficient influence function of $F^a(t)=F_1^a(t)+F_3^a(t)$ is

$$\varphi^a(t)=\varphi_1^a(t)+\varphi_3^a(t).$$

We substitute the models in the efficient influence function with the fitted models. Let $P_n$ be the empirical measure on the observed sample. Solving the estimating equation $P_n\{\widehat{\varphi}^a(t)\}=0$, we obtain $\widetilde{F}^a(t)=P_n\{\widehat{\psi}^a(t)\}$, where

$$\begin{aligned}
\psi^a(t)=&\int_{\mathcal{X}}\int_0^t\exp\{-\Lambda_1^{a_1}(s;x)\}\left\{\frac{I(A=a_1)}{P(A=a_1\mid X)}\frac{dM_1(s;A,X)}{P(\widetilde{T}\wedge\widetilde{R}\geq s\mid A,X)}\right.\\
&\left.-\sum_{j\in\{1,2\}}\frac{I(A=a_j)}{P(A=a_j\mid X)}\int_0^s\frac{dM_j(u;A,X)}{P(\widetilde{T}\wedge\widetilde{R}\geq u\mid A,X)}d\Lambda_1^{a_1}(s;X)\right\}\\
&+\int_{\mathcal{X}}\int_0^t\int_0^s\exp\{-\Lambda_2^{a_2}(r;X)-\Lambda_3^{a_3}(s;r,X)\}\\
&\left\{\frac{I(A=a_2)}{P(A=a_2\mid X)}\frac{dM_2(r;A,X)}{P(\widetilde{T}\wedge\widetilde{R}\geq r)}d\Lambda_3^{a_3}(s;r,X)\right.\\
&-\sum_{j\in\{1,2\}}\frac{I(A=a_j)}{P(A=a_j\mid X)}\int_0^r\frac{dM_j(u;A,X)}{P(\widetilde{T}\wedge\widetilde{R}\geq u\mid A,X)}d\Lambda_2^{a_2}(r;X)d\Lambda_3^{a_3}(s;r,X)\\
&+\frac{I(A=a_3)}{P(A=a_3\mid X)}\frac{dM_3(s;\widetilde{R},A,X)}{P(\mathcal{H}(\widetilde{T},\widetilde{R})\mid A,X)}d\Lambda_2^{a_2}(s;X)\\
&\left.-\frac{I(A=a_3)}{P(A=a_3\mid X)}\int_{\mathcal{H}(s,\widetilde{R})}\frac{dM_3(u;\widetilde{R},A,X)}{P(\mathcal{H}(u,\widetilde{R})\mid A,X)}d\Lambda_2^{a_2}(r;X)d\Lambda_3^{a_3}(s;r,X)\right\}\\
&+F^{(a_1,a_2,a_3)}(t;X).
\end{aligned}$$

Notice that

$$P_n\widehat{\psi}^a(t)=P_n\psi^a(t)+(P-P_n)(\psi^a(t)-\widehat{\psi}^a(t))+P(\widehat{\psi}^a(t)-\psi^a(t)).$$

The first term is as if all models are known. The second term in $o_p(n^{-1/2})$ since $\widehat{\psi}^a(t)$ belongs to a Donsker class. The third term can be bounded by (ignorabing a constant multiplier)

$$\sup_{j\in\{1,2,3\}}E\left[\{\widehat{P}(A=a_j\mid X)-P(A=a_j\mid X)\}\{\widehat{\Lambda}_j^{a_j}(t;\mathcal{F}(t))-\Lambda_j^{a_j}(t;\mathcal{F}(t))\}\right],$$
$$\sup_{j\in\{1,2,3\}}E\left[\{\widehat{\Lambda}_C^{a_j}(t;\mathcal{F}(t))-\Lambda_C^{a_j}(t;\mathcal{F}(t))\}\{\widehat{\Lambda}_j^{a_j}(t;\mathcal{F}(t))-\Lambda_j^{a_j}(t;\mathcal{F}(t))\}\right].$$

By the Cauchy-Schwarz, if all models converge at rate faster than $o_p(n^{-1/2})$, then the third term is $o_p(n^{-1/2})$. Therefore, $P_n\widehat{\psi}^a(t)$ and $P_n\psi^a(t)$ are asymptotic equivalent,

$$\widetilde{F}^a(t)=P_n\widehat{\psi}^a(t)=P_n\psi^a(t)+o_p(n^{-1/2}),$$

and thus

$$n^{1/2}\{\widetilde{F}^a(t)-F^a(t)\}\xrightarrow{d}N\left(0,E[\{\varphi^a(t)\}^2]\right).$$

# F Relaxing random censoring to conditionally random censoring

## F.1 Identification

We first show that the potential censoring probability $S_C^a(t;x) = P(C^a \geq t \mid X = x)$ is identifiable. The hazard of censoring

$$\begin{aligned} d\Lambda_C^a(t;x) &= P(t \leq C^a < t + dt \mid C^a \geq t, X = x) \\ &= P(t \leq C^a < t + dt \mid C^a \geq t, T^a \geq t, X = x) \\ &= P(t \leq C^a < t + dt \mid C^a \geq t, T^a \geq t, A = a, X = x) \\ &= P(t \leq \widetilde{T}^a < t + dt, \delta_T^a = 0 \mid \widetilde{T}^a \geq t, A = a, X = x) \\ &= P(t \leq \widetilde{T} < t + dt, \delta_T = 0 \mid \widetilde{T} \geq t, A = a, X = x). \end{aligned}$$

So

$$S_C^a(t;x) = \exp\left\{-\int_0^t d\Lambda_C^a(s;x)\right\}.$$

Next, we look at $d\Lambda_1^a(t)$. By definition,

$$d\Lambda_1^a(t) = \frac{P(t \leq T^a < t + dt, R^a > t)}{P(T^a \geq t, R^a \geq t)}.$$

For the denominator,

$$\begin{aligned} & E\left\{\frac{I(\widetilde{T} \geq t, \widetilde{R} \geq t, A = a)}{P(A = a \mid X) S_C^a(t;X)}\right\} \\ &= E\left\{\frac{I(\widetilde{T}^a \geq t, \widetilde{R}^a \geq t, A = a)}{P(A = a \mid X) S_C^a(t;X)}\right\} \\ &= E\left\{\frac{I(T^a \geq t, R^a \geq t, C^a \geq t, A = a)}{P(A = a \mid X) S_C^a(t;X)}\right\} \\ &= E\left[E\left\{\frac{I(T^a \geq t, R^a \geq t, C^a \geq t, A = a)}{P(A = a \mid X) S_C^a(t;X)} \,\Big|\, T^a, R^a, C^a, X\right\}\right] \\ &= E\left\{\frac{I(T^a \geq t, R^a \geq t, C^a \geq t) P(A = a \mid T^a, R^a, C^a, X)}{P(A = a \mid X) S_C^a(t;X)}\right\} \\ &= E\left\{\frac{I(T^a \geq t, R^a \geq t, C^a \geq t)}{S_C^a(t;X)}\right\} \\ &= E\left[E\left\{\frac{I(T^a \geq t, R^a \geq t, C^a \geq t)}{S_C^a(t;X)} \,\Big|\, T^a, R^a, X\right\}\right] \\ &= E\left\{\frac{I(T^a \geq t, R^a \geq t) P(C^a \geq t \mid T^a,^a, X)}{S_C^a(t;X)}\right\} \\ &= E\left\{I(T^a \geq t, R^a \geq t)\right\} \\ &= P(T^a \geq t, R^a \geq t). \end{aligned}$$

For the numerator, similarly,

$$E\left\{\frac{I(t \leq \widetilde{T} < t + dt, \widetilde{R} \geq t, A = a)}{P(A = a \mid X) S_C^a(t;X)}\right\} = P(t \geq T^a < t + dt, R^a \geq t).$$

This proves the identifiability of $d\Lambda_1^a(t)$.

We can show

$$d\Lambda_2^a(t) = \frac{E\{I(t \le \widetilde{R} < t+dt, \delta_R = 1 \mid A = a)/P(A = a \mid X)S_C^a(t;X)\}}{E\{I(\widetilde{T} \ge t, \widetilde{R} \ge t, A = a)/P(A = a \mid X)S_C^a(t;X)\}},$$

$$d\Lambda_3^a(t;r) = \frac{E\{I(t \le \widetilde{T} < t+dt, \widetilde{R} = r, \delta_T\delta_R = 1, A = a)/P(A = a_3 \mid X)S_C^a(t;X)\}}{E\{I(\widetilde{T} \ge t, \widetilde{R} = r, \delta_R = 1, A = a)/P(A = a \mid X)S_C^a(t;X)\}}.$$

in the same manner.

## F.2 Estimation

Define weights

$$w_i(t;a_j) = \frac{I(A_i = a_j)}{P(A_i = a_j \mid X_i)S_C^a(t;X_i)},\ j = 1,2,3.$$

In the definition of weighted counting processes, at-risk processes and martingales, the weights $w_i(a_j)$ should be replaced with $w_i(t;a_j)$. Now the filters become

$$\mathcal{F}_j^{a_j}(t) = \{Y_{ij}(s;a_j).w_i(s;a_j) : s \le t, i = 1,\dots,n\}$$

for $j = 1,2$.

However, the filter could be more complicated for the transition process from State 2 to State 3. Under Markov assumption, the filter is

$$\mathcal{F}_3^{a_3}(t) = \{Y_{i3}(s;a_3).w_i(s;a_3) : s \le t, i = 1,\dots,n\}.$$

Under semi-Markov assumption, note that

$$\begin{aligned} d\Lambda_3^{a_3}(t;r) &= P(t \le T^{a_3} < t+dt \mid T^{a_3} \ge t, R^{a_3} = r) \\ &= P(u \le T^{a_3} - R^{a_3} < u+du \mid T^{a_3} - R^{a_3} \ge u, R^{a_3} = r) \\ &= P(u \le T^{a_3} - R^{a_3} < u+du \mid T^{a_3} - R^{a_3} \ge u) \end{aligned}$$

because the expression should be irrelevant to $r$ given $u = t - r$. Here we need an additional rank preservation assumption for the censoring

$$P(C^{a_3} \ge t \mid X) = P(C^{a_3} \ge u \mid X)h(t,u,a_3),$$

where $h(t,u,a_3)$ is an arbitrary (unknown) function, so that

$$\begin{aligned} d\Lambda_3^{a_3}(t;r) &= \frac{E\{I(u \le T^{a_3} - R^{a_3} < u+du, C^{a_3} - R^{a_3} \ge u)/P(A = a_3 \mid X)S_C^{a_3}(t;X)\}}{E\{I(T^{a_3} - R^{a_3} \ge u, C^{a_3} - R^{a_3} \ge u)/P(A = a_3 \mid X)S_C^{a_3}(t;X)\}} \\ &= \frac{E\{I(u \le T^{a_3} - R^{a_3} < u+du, C^{a_3} - R^{a_3} \ge u)/P(A = a_3 \mid X)S_C^{a_3}(u;X)\}}{E\{I(T^{a_3} - R^{a_3} \ge u, C^{a_3} - R^{a_3} \ge u)/P(A = a_3 \mid X)S_C^{a_3}(u;X)\}}. \end{aligned}$$

Only with the rank preservation, we can treat $T^a - R^a$ as a time-to-event outcome with conditionally random censoring, and thus the filter

$$\mathcal{F}_3^{a_3}(t) = \{Y_{i3}(s;a_3).w_i(s;a_3) : s \le t, i = 1,\dots,n\}.$$

# G Partial dismissible components with time-varying covariates

In the presence of time-varying covariates $X(t)$, we let $\mathcal{F}^-(t) = \{X(s), S(s) : s < t\}$ be the information prior to time $t$ including time-varying covariates and prior statuses, and $\mathcal{F}(t) = \mathcal{F}^-(t) \cup X(t)$. Let $\lambda_j^a(t; \mathcal{F}(t))$ be the hazard of transiting to State $j \in \{1, 2, 3\}$ conditional on the information $\mathcal{F}(t)$ under the hypothetical treatment $a = (a_1, a_2, a_3)$. As an alternative to full isolation in Assumption 5, we consider the dismissible components conditional on the information $\mathcal{F}(t)$ as follows:

$$\lambda_j^a(t; \mathcal{F}(t)) = \lambda_j^{a_j}(t; \mathcal{F}(t)) = \lambda_j(t; a_j, \mathcal{F}(t)), \ \forall\ 0 \le t \le \tau,\ j = 1, 2, 3. \tag{2}$$

This assumption means that the effect of $A_j = a_j$ on the hazards $\lambda_j^{(a_1,a_2,a_3)}(t; \mathcal{F}(t))$ can be blocked by conditioning on observed time-varying covariates and status information in $\mathcal{F}(t)$. Cross-world dependence is precluded. Write $\Lambda_j^a(t; \mathcal{F}(t)) = \int_0^t \lambda_j^a(s; \mathcal{F}(s)) ds$.

In addition, to relax random censoring (Assumption 3), we assume that the hazard of censoring does not depend on future information,

$$I(t \le C^a < t^+) \perp\!\!\!\perp \mathcal{F}(u) \mid A = a, \mathcal{F}(t),\ u > t,\ \forall\ 0 \le t \le \tau. \tag{3}$$

So we can write the hazard of censoring

$$\lambda_C(t; a_j, \mathcal{F}(t)) = \lim_{dt \to 0} \frac{1}{dt} P(t \le C < t + dt \mid A = a_j, C \ge t, \mathcal{F}(t)),\ j = 1, 2, 3.$$

Write $\Lambda_C(t; a_j, \mathcal{F}(t)) = \int_0^t \lambda_C(s; a_j, \mathcal{F}(s)) dt$. Thus, the hazard of transition $\lambda_j(t; a_j, \mathcal{F}(t))$ and the hazard of censoring $\lambda_C(t; a_j, \mathcal{F}(t))$ can be identified in the $A = a_j$ treatment group whenever there are observed data with information $\mathcal{F}(t)$, i.e., strong positivity

$$p(\mathcal{F}(t)) > 0 \Rightarrow p(\mathcal{F}(t) \mid A) \cdot P(C^A > t \mid A, \mathcal{F}(t)) > 0,\ \forall\ 0 \le t \le \tau, \tag{4}$$

where $p(\mathcal{F}(t) \mid A)$ is the density of $\mathcal{F}(t)$ in the $A$ treatment group defined on $\mathcal{X}(t)$, the the support of $\mathcal{F}(t)$ under the hypothetical treatments $\{a = (a_1, a_2, a_3) : a_1, a_2, a_3 = 0, 1\}$.

Next, we assume that the time-varying covariates $X(t)$ consist of an $A_1$-related part $X_1(t)$, an $A_2$-related part $X_2(t)$ and an $A_3$-related part $X_3(t)$, with dismissible components

$$p(X_1(t) \mid A = (a_1, a_2, a_3), \mathcal{F}^-(t)) = p(X_1(t) \mid A = a_1, \mathcal{F}^-(t)), \tag{5}$$
$$p(X_2(t) \mid A = (a_1, a_2, a_3), \mathcal{F}^-(t), X_1(t)) = p(X_2(t) \mid A = a_2, \mathcal{F}^-(t), X_1(t)), \tag{6}$$
$$p(X_3(t) \mid A = (a_1, a_2, a_3), \mathcal{F}^-(t), X_1(t), X_2(t)) = p(X_3(t) \mid A = a_3, \mathcal{F}^-(t), X_1(t), X_2(t)), \tag{7}$$

where $p(\cdot|\cdot)$ means conditional density. Let $S_j(t)$ be the indicator function of whether a unit is in State $j$ at time $t$. The conditional densities above indicate that we have ordered the information at time $t$ in the order $(X_1(t), X_2(t), X_3(t), S_1(t), S_2(t), S_3(t))$. So we can denote the transition density of covariates $X(t)$ at time $t$ under the hypothetical treatment $a = (a_1, a_2, a_3)$ by

$$\begin{aligned} p(X(t); a, \mathcal{F}^-(t)) = p(X_1(t) \mid A = a_1, \mathcal{F}^-(t)) \cdot p(X_2(t) \mid A = a_2, \mathcal{F}^-(t), X_1(t)) \\ \cdot\, p(X_3(t) \mid A = a_3, \mathcal{F}^-(t), X_1(t), X_2(t)). \end{aligned}$$

Although the transition density of covariates is defined everywhere in $[0, \tau]$, the time-varying covariates may only change values at some discrete time points. If $X(t)$ does not vary at time $t$, then $p(X(t); a, \mathcal{F}^-(t)) = 1$ on $X(t)$. The counterfactual cumulative incidences can be identified by a continuous generalization of g-formula (Robins, 1997; Robins and Richardson, 2010; Young et al., 2020; Stensrud et al., 2022).

**Theorem S2.** *Under consistency (Assumption 1), ingorability (Assumption 2), timewise random censoring (Condition* (3)*), strong positivity (Conditon* (4)*) and partial dismisible treatment components (Conditions* (2) *and* (5)*–*(7)*), the counterfactual cumulative incidences of States 1, 2 and 3 are*

$$
\begin{aligned}
F_1^{(a_1,a_2,a_3)}(t) &= \int_0^t \int_{\{\mathcal{X}(u)\}_0^s} \exp\{-\Lambda_1(s; a_1, \mathcal{F}(s)) - \Lambda_2(s; a_2, \mathcal{F}(s))\}\lambda_1(s; a_1, \mathcal{F}(s)) \\
&\qquad \prod_0^s \{p(y; a, \mathcal{F}^-(u))dy\}ds, \\
F_2^{(a_1,a_2,a_3)}(t) &= \int_0^t \int_{\{\mathcal{X}(u)\}_0^s} \exp\{-\Lambda_1(s; a_1, \mathcal{F}(s)) - \Lambda_2(s; a_2, \mathcal{F}(s))\}\lambda_2(s; a_2, \mathcal{F}(s)) \\
&\qquad \prod_0^s \{p(y; a, \mathcal{F}^-(u))dy\}ds, \\
F_3^{(a_1,a_2,a_3)}(t) &= F_2^{(a_1,a_2,a_3)}(t) - \int_0^t \int_{\{\mathcal{X}(u)\}_0^s} \exp\{-\Lambda_1(s; a_1, \mathcal{F}(s)) - \Lambda_2(s; a_2, \mathcal{F}(s)) \\
&\qquad - \Lambda_3(t; a_3, \mathcal{F}(t)) + \Lambda_3(s; a_3, \mathcal{F}(s))\}\lambda_2(s; a_2, \mathcal{F}(s)) \prod_0^s \{p(y; a, \mathcal{F}^-(u))dy\}ds.
\end{aligned}
$$

Another way to identify the counterfactual cumulative incidences is by weighting. Let

$$
\begin{aligned}
W_1(t; j, a, a_k) &= \frac{\exp\{-\Lambda_j(t; a_j, \mathcal{F}(t)\}}{\exp\{-\Lambda_j(t; a_k, \mathcal{F}(t)\}}, \\
W_2(t; a, a_k) &= \prod_0^t \left\{ \frac{P(A = a_1 \mid X_1(t), \mathcal{F}^-(s))}{P(A = a_k \mid X_1(t), \mathcal{F}^-(s))} \frac{P(A = a_k \mid \mathcal{F}^-(s))}{P(A = a_1 \mid \mathcal{F}^-(s))} \right. \\
&\quad \cdot \frac{P(A = a_2 \mid X_1(s), X_2(s), \mathcal{F}^-(s))}{P(A = a_k \mid X_1(s), X_2(s)\mathcal{F}^-(s))} \frac{P(A = a_k \mid X_1(s), \mathcal{F}^-(s))}{P(A = a_2 \mid X_1(s), \mathcal{F}^-(s))} \\
&\quad \left. \cdot \frac{P(A = a_3 \mid X_1(s), X_2(s), X_3(s), \mathcal{F}^-(s))}{P(A = a_k \mid X_1(s), X_2(s), X_3(s)\mathcal{F}^-(s))} \frac{P(A = a_k \mid X_2(s), X_3(s), \mathcal{F}^-(s))}{P(A = a_3 \mid X_2(s), X_3(s), \mathcal{F}^-(s))} \right\}, \\
W_3(t; a_k) &= \frac{I(A = a_k)}{\exp\{-\Lambda_C(t; a_k, \mathcal{F}(t))\}}.
\end{aligned}
$$

Since we would only use data from a single group $A = a_k$ to estimate the counterfactual hazard under the hypothetical treatment $A = a$, we rely on the weight $W_1(t; j, a, a_k)$ to correct for the cause-specific hazards, $W_2(t; a, a_k)$ to correct for the distribution of time-varying covariates, and $W_3(t; a_k)$ to correct for censoring. When the time-varying covariates change values at finite time points, then $W_2(t; a, a_k)$ is the product with terms evaluated at those time points.

**Theorem S3.** *Under consistency (Assumption 1), ingorability (Assumption 2), timewise random censoring (Condition* (3)*), strong positivity (Conditon* (4)*) and partial dismisible treatment components (Conditions* (2) *and* (5)*–*(7)*), the counterfactual cumulative incidences of States 1, 2 and 3 are*

$$
\begin{aligned}
F_1^{(a_1,a_2,a_3)}(t) = E\bigg[ \int_0^t & W_1(s; 2, a, a_1) W_2(s; a, a_1) W_3(s; a_1) \\
& \cdot I(s \leq \widetilde{T} < s + ds, \delta_T(1 - \delta_R) = 1) \mid A = a_1 \bigg],
\end{aligned}
$$

$$F_2^{(a_1,a_2,a_3)}(t) = E\bigg[\int_0^t W_1(s;1,a,a_2)W_2(s;a,a_2)W_3(s;a_2)I(s \le \widetilde{R} < s+ds, \delta_R = 1) \mid A = a_2\bigg],$$

$$F_3^{(a_1,a_2,a_3)}(t) = F_2^{(a_1,a_2,a_3)}(t) - E\bigg[\int_0^t W_1(s;1,a,a_2)W_1(t;3,a,a_2)W_1(s;3,a,a_2)^{-1} \cdot W_2(s;a,a_2)W_3(s;a_2)I(s \le \widetilde{T} < s+ds, \delta_T\delta_R = 1) \mid A = a_2\bigg].$$

These cumulative incidences can be estimated by plug-in estimators using parametric modelling.

We only prove the identification result for $F_1^{(a_1,a_2,a_3)}(t)$. Let $S_{12}(t;a,\mathcal{F}(t)) = P(T^a \ge t, R^a \ge t \mid A = a, \mathcal{F}(t))$ be the survival function of $\min\{T^a, R^a\}$ conditional on prior information $\mathcal{F}(t)$ in the $A = a$ treatment group. Observe that the conditional density of $\min\{T^a, R^a\}$ at time $t$

$$-\frac{d}{dt}S_{12}(t;a,\mathcal{F}(t)) = S_{12}(t;a,\mathcal{F}(t)) \cdot \{\lambda_1(t;a,\mathcal{F}(t)) + \lambda_2(t;a,\mathcal{F}(t))\},$$

So $S_{12}(t;a,\mathcal{F}(t)) = \exp\{-\Lambda_1(t;a,\mathcal{F}(t)) - \Lambda_2(t;a,\mathcal{F}(t))\}$. Let $S_C(t;a,\mathcal{F}(t)) = P(C^a \ge t \mid A = a, \mathcal{F}(t))$ be the survival function of censoring conditional on prior information $\mathcal{F}(t)$ in the $A = a$ treatment group. Observe that the conditional density of censoring at time $t$

$$-\frac{d}{dt}S_C(t;a,\mathcal{F}(t)) = S_C(t;a,\mathcal{F}(t)) \cdot \lambda_C(t;a,\mathcal{F}(t)),$$

So $S_C(t;a,\mathcal{F}(t)) = \exp\{-\Lambda_C(t;a,\mathcal{F}(t))\}$. Note the weight $W_2(t;a,a_k)$ generates the ratio of covariates transition rates under different treatments,

$$\frac{p(X_1(t) \mid A = a_1, \mathcal{F}^-(t))}{p(X_1(t) \mid A = a_k, \mathcal{F}^-(t))} = \frac{P(A = a_1 \mid X_1(t), \mathcal{F}^-(t))}{P(A = a_k \mid X_1(t), \mathcal{F}^-(t))} \cdot \frac{P(A = a_k \mid \mathcal{F}^-(t))}{P(A = a_1 \mid \mathcal{F}^-(t))},$$

$$\frac{p(X_2(t) \mid A = a_2, X_1(t), \mathcal{F}^-(t))}{p(X_2(t) \mid A = a_k, X_1(t), \mathcal{F}^-(t))} = \frac{P(A = a_2 \mid X_1(t), X_2(t), \mathcal{F}^-(t))}{P(A = a_k \mid X_1(t), X_2(t), \mathcal{F}^-(t))} \cdot \frac{P(A = a_k \mid X_1(t), \mathcal{F}^-(t))}{P(A = a_2 \mid X_1(t), \mathcal{F}^-(t))},$$

$$\frac{p(X_3(t) \mid A = a_3, X_1(t), X_2(t), \mathcal{F}^-(t))}{p(X_3(t) \mid A = a_k, X_1(t), X_2(t), \mathcal{F}^-(t))} = \frac{P(A = a_3 \mid X_1(t), X_2(t), X_3(t), \mathcal{F}^-(t))}{P(A = a_k \mid X_1(t), X_2(t), X_3(t), \mathcal{F}^-(t))} \cdot \frac{P(A = a_k \mid X_1(t), X_2(t), \mathcal{F}^-(t))}{P(A = a_3 \mid X_1(t), X_2(t), \mathcal{F}^-(t))}.$$

So

$$W_2(t;a,a_k) = \prod_0^t \frac{p(X(t) \mid A = a, \mathcal{F}^-(t))}{p(X(t) \mid A = a_k, \mathcal{F}^-(t))}.$$

Let

$$f_1(t;a,\mathcal{F}(s)) := \lim_{dt \to 0} \frac{1}{dt} P(t \le T^a < t+dt, R^a > t \mid A = a, \mathcal{F}(s))$$

be the conditional density of State 1 given the information prior to $s$ in the $A = a$ treatment group. By ignorability,

$$f_1(t;a) := \lim_{dt \to 0} \frac{1}{dt} P(t \le T^a < t+dt, R^a > t \mid A = a) = \lim_{dt \to 0} \frac{d}{dt} F_1^a(t).$$

Now we prove the weighted identification formula. To prove, we first calculate the conditional expectation given $\mathcal{F}(t)$, then $\mathcal{F}^-(t)$, and so on until $\mathcal{F}^-(0) = \{X(0)\}$ in the $A = a_1$ treatment group.

$$
\begin{aligned}
&E\Big[\int_0^t \frac{e^{-\Lambda_2(s;a_2,\mathcal{F}(s))}}{e^{-\Lambda_2(s;a_1,\mathcal{F}(s))}} \prod_0^t \frac{p(X(s) \mid A=a,\mathcal{F}^-(s))}{p(X(s) \mid A=a_1,\mathcal{F}^-(s))} \frac{I(A=a_1)}{e^{-\Lambda_C(s;a_1,\mathcal{F}(s))}} \\
&\quad \cdot I(s \le \widetilde{T} < s+ds, \delta_T(1-\delta_R)=1) \mid A=a_1\Big] \\
&= E\Big[\int_0^t \frac{e^{-\Lambda_2(s;a_2,\mathcal{F}(s))}}{e^{-\Lambda_2(s;a_1,\mathcal{F}(s))}} \prod_0^t \frac{p(X(s) \mid A=a,\mathcal{F}^-(s))}{p(X(s) \mid A=a_1,\mathcal{F}^-(s))} \frac{I(A=a_1)}{e^{-\Lambda_C(s;a_1,\mathcal{F}(s))}} \\
&\quad \cdot P(T^{a_1} \ge s, R^{a_1} \ge s, C^{a_1} \ge s \mid A=a_1,\mathcal{F}(s))\lambda_1(s;a_1,\mathcal{F}(s))ds \mid A=a_1\Big] \\
&= E\Big[\int_0^t \frac{e^{-\Lambda_2(s;a_2,\mathcal{F}(s))}}{e^{-\Lambda_2(s;a_1,\mathcal{F}(s))}} \prod_0^t \frac{p(X(s) \mid A=a,\mathcal{F}^-(s))}{p(X(s) \mid A=a_1,\mathcal{F}^-(s))} \frac{I(A=a_1)}{e^{-\Lambda_C(s;a_1,\mathcal{F}(s))}} \\
&\quad \cdot P(T^{a_1} \ge s, R^{a_1} \ge s \mid A=a_1,\mathcal{F}(s))P(C^{a_1} \ge s \mid A=a_1,\mathcal{F}(s))\lambda_1(s;a_1,\mathcal{F}(s))ds \mid A=a_1\Big] \\
&= E\Big[\int_0^t \frac{e^{-\Lambda_2(s;a_2,\mathcal{F}(s))}}{e^{-\Lambda_2(s;a_1,\mathcal{F}(s))}} \prod_0^t \frac{p(X(s) \mid A=a,\mathcal{F}^-(s))}{p(X(s) \mid A=a_1,\mathcal{F}^-(s))} \\
&\quad \cdot P(T^{a_1} \ge s, R^{a_1} \ge s \mid A=a_1,\mathcal{F}(s))\lambda_1(s;a_1,\mathcal{F}(s))ds \mid A=a_1\Big] \\
&= E\Big[\int_0^t \frac{e^{-\Lambda_2(s;a_2,\mathcal{F}(s))}}{e^{-\Lambda_2(s;a_1,\mathcal{F}(s))}} \prod_0^t \frac{p(X(s) \mid A=a,\mathcal{F}^-(s))}{p(X(s) \mid A=a_1,\mathcal{F}^-(s))} \\
&\quad \cdot e^{-\Lambda_1(s;a_1,\mathcal{F}(s))-\Lambda_2(s;a_1,\mathcal{F}(s))}\lambda_1(s;a_1,\mathcal{F}(s))ds \mid A=a_1\Big] \\
&= E\Big[\int_0^t \prod_0^t \frac{p(X(s) \mid A=a,\mathcal{F}^-(s))}{p(X(s) \mid A=a_1,\mathcal{F}^-(s))} e^{-\Lambda_1(s;a_1,\mathcal{F}(s))-\Lambda_2(s;a_2,\mathcal{F}(s))}\lambda_1(s;a_1,\mathcal{F}(s))ds \mid A=a_1\Big] \\
&= E\Big[\int_0^t \prod_0^t \frac{p(X(s) \mid A=a,\mathcal{F}^-(s))}{p(X(s) \mid A=a_1,\mathcal{F}^-(s))} P(T^a \ge s, R^a \ge s \mid A=a,\mathcal{F}(s))\lambda_1(s;a_1,\mathcal{F}(s))ds \mid A=a_1\Big] \\
&= E\Big[\int_0^t \int_{\mathcal{X}(s)} \prod_0^t \frac{p(X(s) \mid A=a,\mathcal{F}^-(s))}{p(X(s) \mid A=a_1,\mathcal{F}^-(s))} P(T^a \ge s, R^a \ge s \mid A=a,\mathcal{F}(s))\lambda_1(s;a_1,\mathcal{F}(s)) \\
&\quad \cdot p(X(s) \mid A=a_1,\mathcal{F}^-(s))dX(s)ds \mid A=a_1\Big] \\
&= E\Big[\int_0^t \prod_0^{t^-} \frac{p(X(s) \mid A=a,\mathcal{F}^-(s))}{p(X(s) \mid A=a_1,\mathcal{F}^-(s))} \int_{\mathcal{X}(s)} P(T^a \ge s, R^a \ge s \mid A=a,\mathcal{F}(s))\lambda_1(s;a_1,\mathcal{F}(s)) \\
&\quad \cdot p(X(s) \mid A=a,\mathcal{F}^-(s))dX(s)ds \mid A=a_1\Big] \\
&= E\Big[\int_0^t \prod_0^{t^-} \frac{p(X(s) \mid A=a,\mathcal{F}^-(s))}{p(X(s) \mid A=a_1,\mathcal{F}^-(s))} f_1(s;a,\mathcal{F}^-(s))ds \mid A=a_1\Big]
\end{aligned}
$$

$$= E\left[\int_0^t \frac{p(X(0)\mid A=a)}{p(X(0)\mid A=a_1)} f_1(s;a,X(0))ds \mid A=a_1\right]$$
$$= E\left[\int_0^t f_1(s;a,X(0))ds \mid A=a\right]$$
$$= \int_0^t f_1(s;a) = F_1^a(t).$$

If there are no post-treatment time-varying covariates, the identification is trivial since $\mathcal{F}(t) = \mathcal{F}(0) = X$ is just the baseline covariates. Specially, **?** derived the efficient influence function under the dismissible components with baseline covariates (but in their work they only decomposed the treatment into two components).

# H Additional simulation results

## H.1 Estimated cumulative incidences and bias

We follow the data generating process in the main paper. To see the performance of estimates, we consider the GNAIPW (Markov), GNAIPW (semi-Markov) and EIF-based estimator. In the EIF-based estimator, we use the Cox proportional hazards model to fit the cause-specific hazards. Figure S2–S4 show the estimated cumulative incidences of $F^{(0,0,0)}(t)$, $F^{(1,0,0)}(t)$ and $F^{(1,0,1)}(t)$, respectively, when the sample size $n = 100$. Figure S5–S7 show the estimated cumulative incidences of $F^{(0,0,0)}(t)$, $F^{(1,0,0)}(t)$ and $F^{(1,0,1)}(t)$, respectively, when the sample size $n = 500$. With a larger sample size, the estimates show smaller variation.

Next, we compare the bias of our proposed estimators (GNAIPW and EIF-based estimator) to the competing method proposed in Huang (2021). We did not perform covariates adjustment in the method of Huang (2021) since the original method did not provide easy-to-implement approach to adjust covariates. Two measures of bias are considered, namely the pointwise bias of estimated cumulative incidences and the (negative) bias of estimated restricted mean survival time (RMST) by integrating the pointwise bias within $[0, t]$, given by

$$E\{\widehat{F}^{(a_1,a_2,a_3)}(t) - F^{(a_1,a_2,a_3)}(t)\},\ E\left[\int_0^t \{\widehat{F}^{(a_1,a_2,a_3)}(s) - F^{(a_1,a_2,a_3)}(s)\}ds\right],$$

respectively. Suppose the sample size $n = 500$. The empirical bias is shown in Figure S8.

When the assumption on $d\Lambda_3^a(t;r)$ is correctly specified (i.e., Setting 1), biases of both proposed methods are very small. Some but small bias is observed when the assumption on $d\Lambda_3^a(t;r)$ is misspecified (i.e., semi-Markov estimators under Setting 2 and Markov estimators under Setting 3). The EIF-based estimator presumes Markovness but has roubustness, so the bias is small in these three settings. However, the EIF-based estimator involves many models. These models are estimated with uncertainty. The EIF-based estimator may show some finite-sample bias. Huang (2021)'s method shows slight bias when estimating $F^{(0,0,0)}(t)$ because the world of $(0,0,0)$ is observable. Huang's method fails to estimate $F^{(1,0,0)}(t)$ because it cannot generate this counterfactual scenario.

## H.2 Empirical assessments of confidence intervals

Let the sample size $n \in \{100, 500\}$. We generate the datasets under the three settings in the main paper for 1000 times. Tables S1–S3 show the empirical coverage rate and width of the 95% pointwise confidence intervals obtained by asymptotic formula at some fixed time points, for

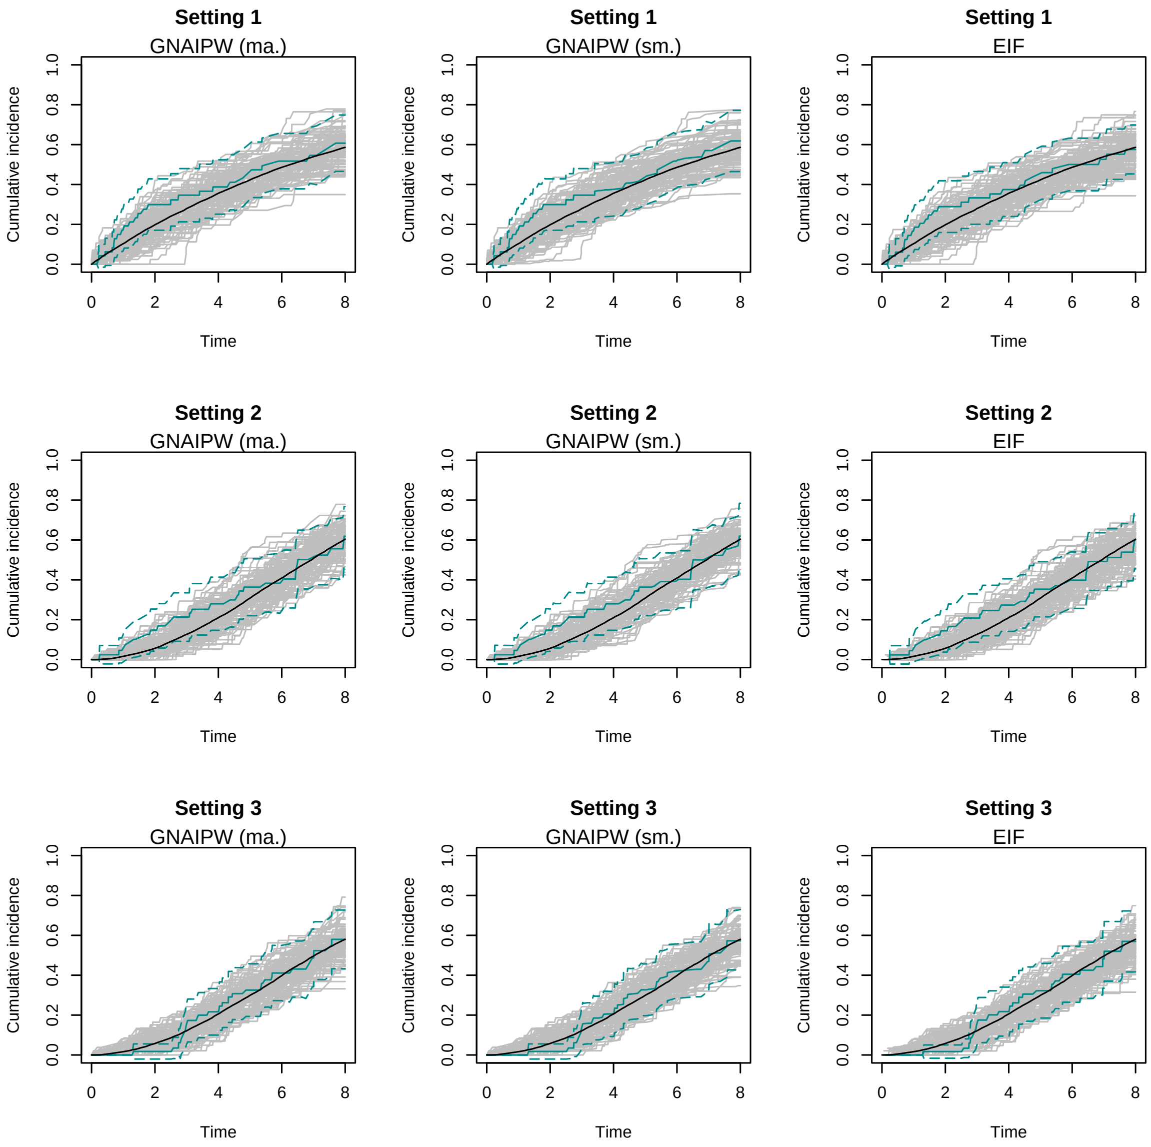


Figure S2: Estimated cumulative incidence functions for $F^{(0,0,0)}(t)$ when $n = 100$. In each panel, the black line is the true incidence, each grey line is an estimated incidence, the solid cyan line is a randomly chosen estimated incidence, and dashed cyan lines denote the 95% asymptotic confidence interval.

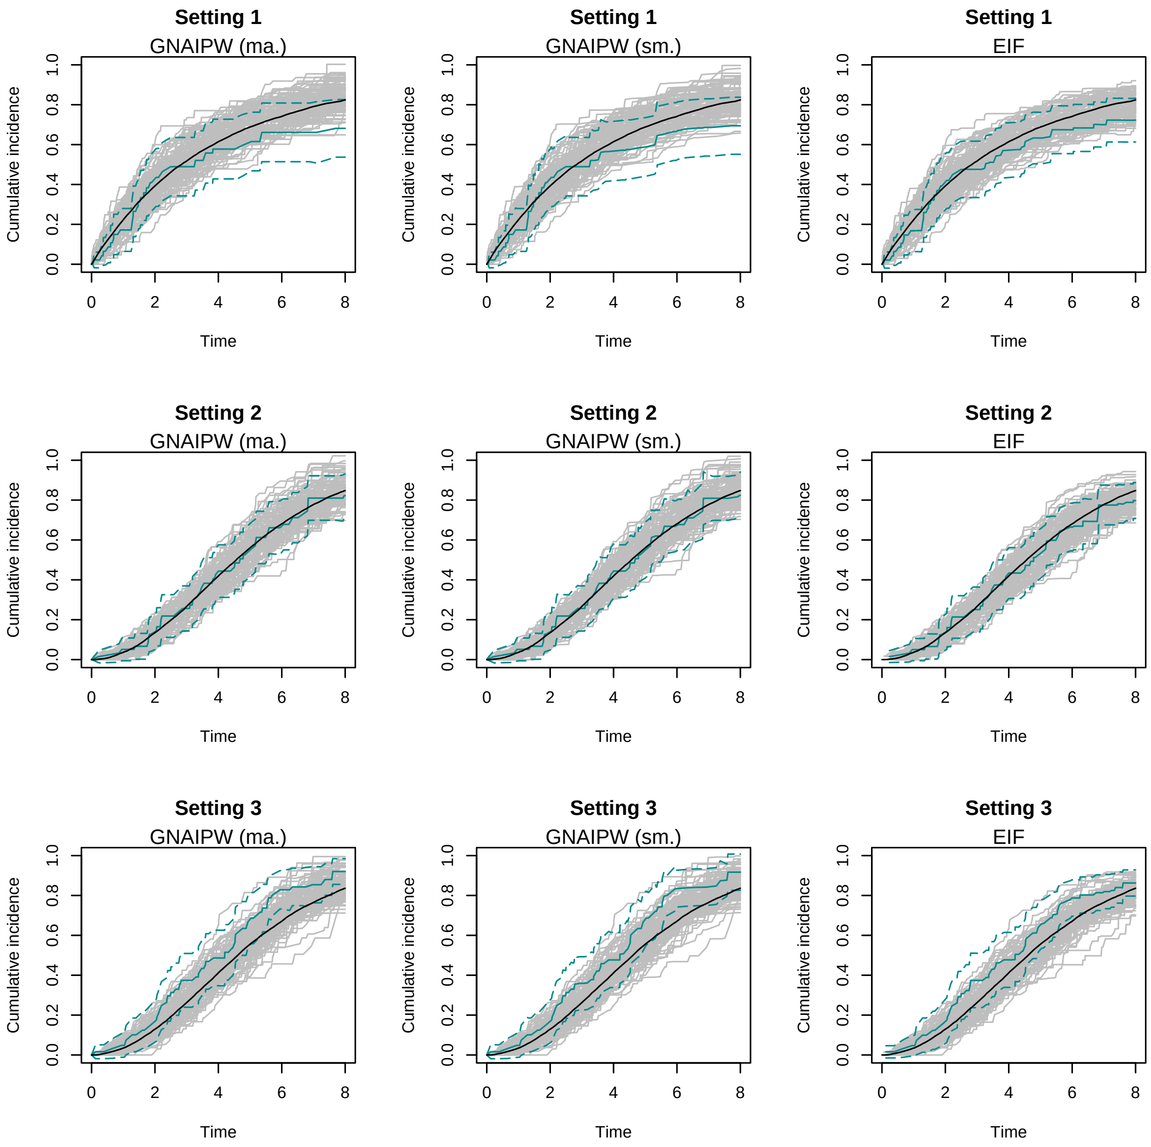


Figure S3: Estimated cumulative incidence functions for $F^{(1,0,0)}(t)$ when $n = 100$. In each panel, the black line is the true incidence, each grey line is an estimated incidence, the solid cyan line is a randomly chosen estimated incidence, and dashed cyan lines denote the 95% asymptotic confidence interval.

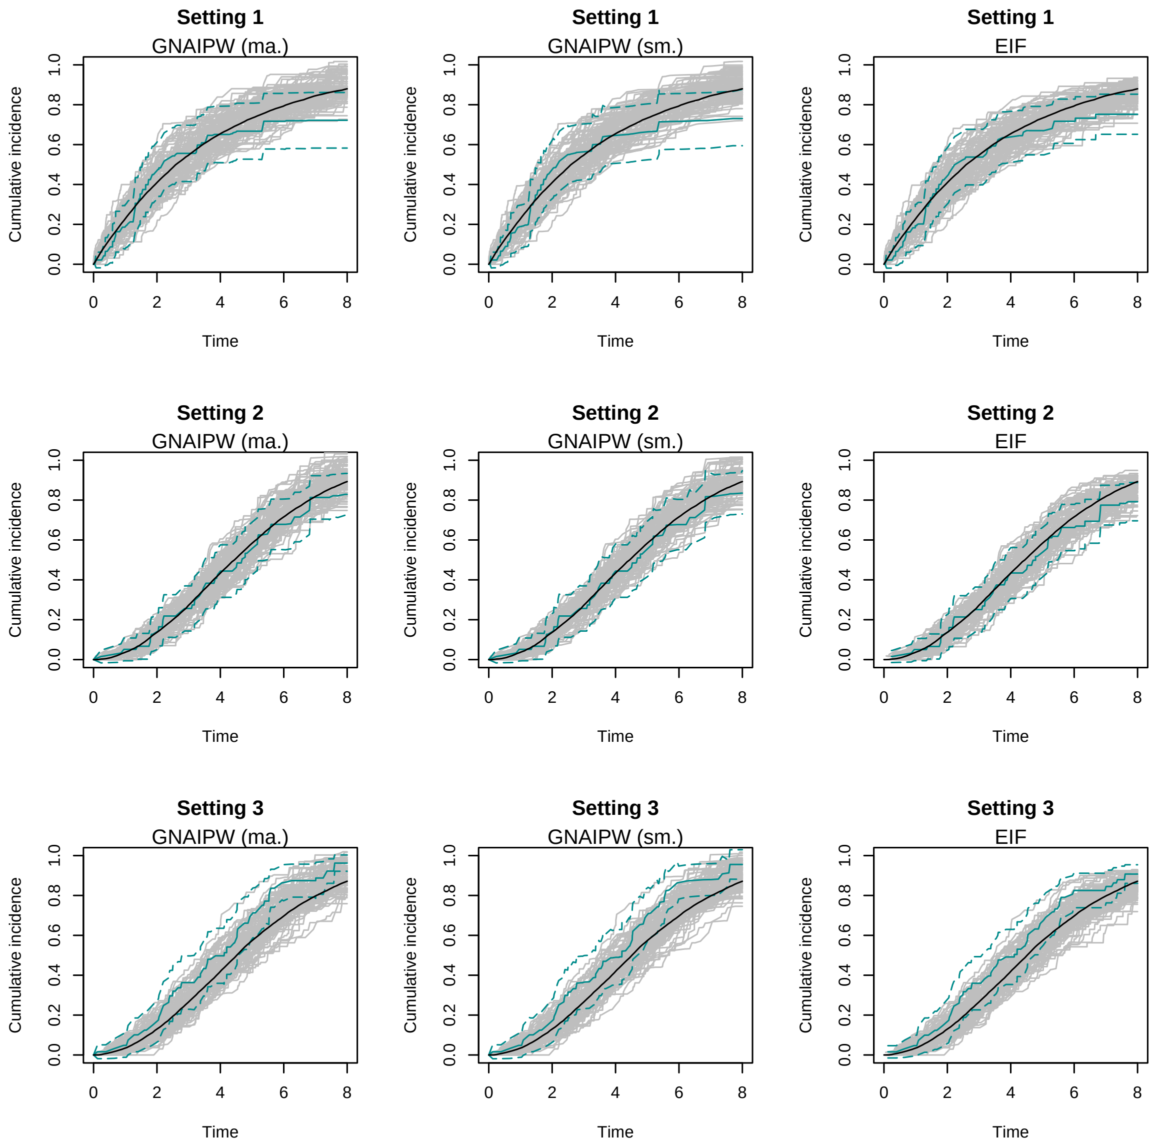


Figure S4: Estimated cumulative incidence functions for $F^{(1,0,1)}(t)$ when $n = 100$. In each panel, the black line is the true incidence, each grey line is an estimated incidence, the solid cyan line is a randomly chosen estimated incidence, and dashed cyan lines denote the 95% asymptotic confidence interval.

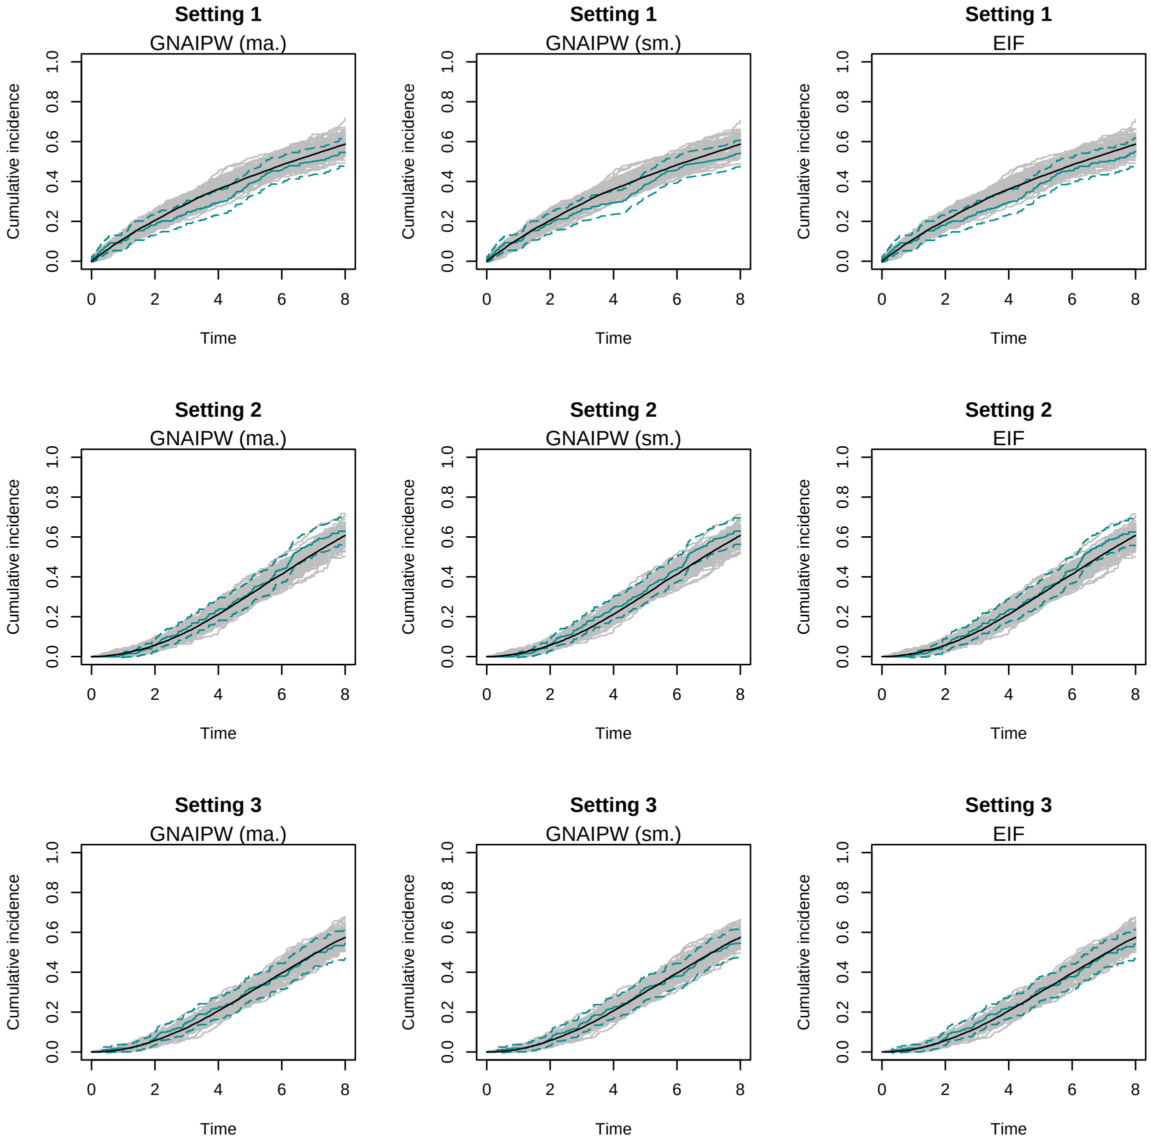


Figure S5: Estimated cumulative incidence functions for $F^{(0,0,0)}(t)$ when $n = 500$. In each panel, the black line is the true incidence, each grey line is an estimated incidence, the solid cyan line is a randomly chosen estimated incidence, and dashed cyan lines denote the 95% asymptotic confidence interval.

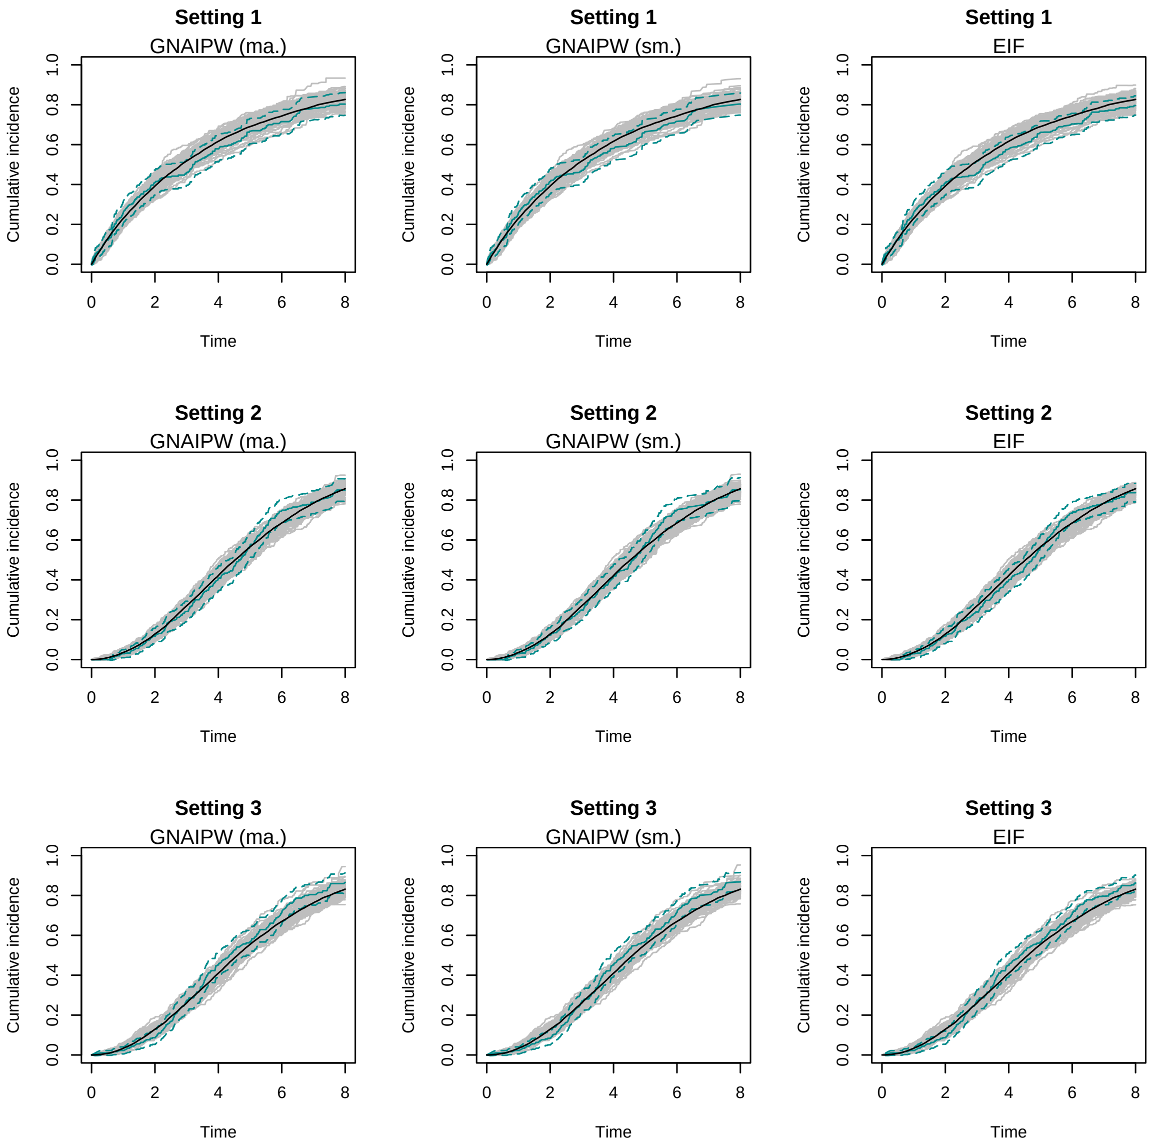


Figure S6: Estimated cumulative incidence functions for $F^{(1,0,0)}(t)$ when $n = 500$. In each panel, the black line is the true incidence, each grey line is an estimated incidence, the solid cyan line is a randomly chosen estimated incidence, and dashed cyan lines denote the 95% asymptotic confidence interval.

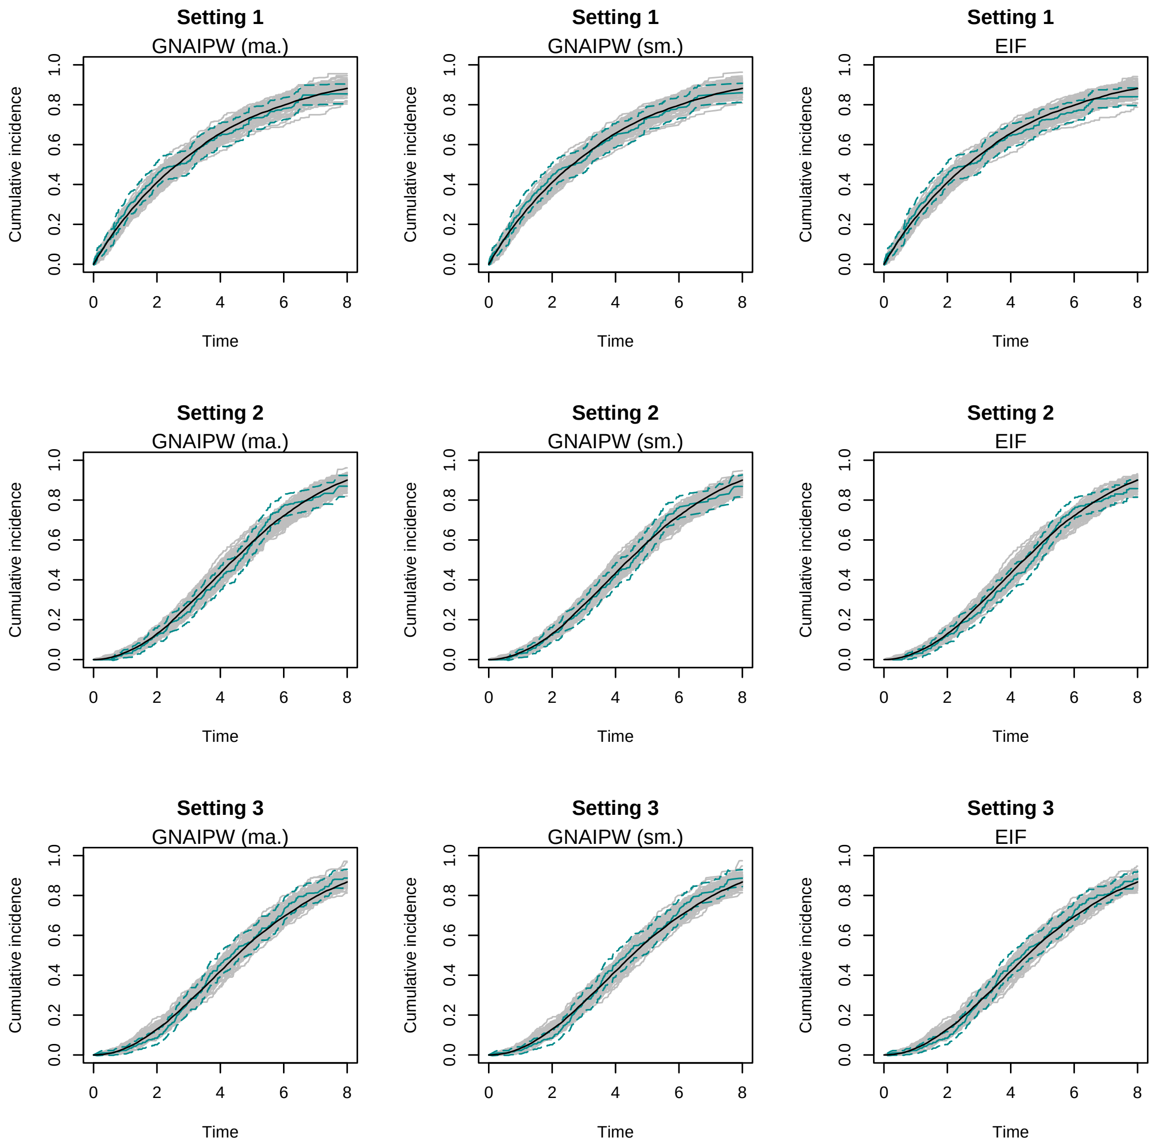


Figure S7: Estimated cumulative incidence functions for $F^{(1,0,1)}(t)$ when $n = 500$. In each panel, the black line is the true incidence, each grey line is an estimated incidence, the solid cyan line is a randomly chosen estimated incidence, and dashed cyan lines denote the 95% asymptotic confidence interval.

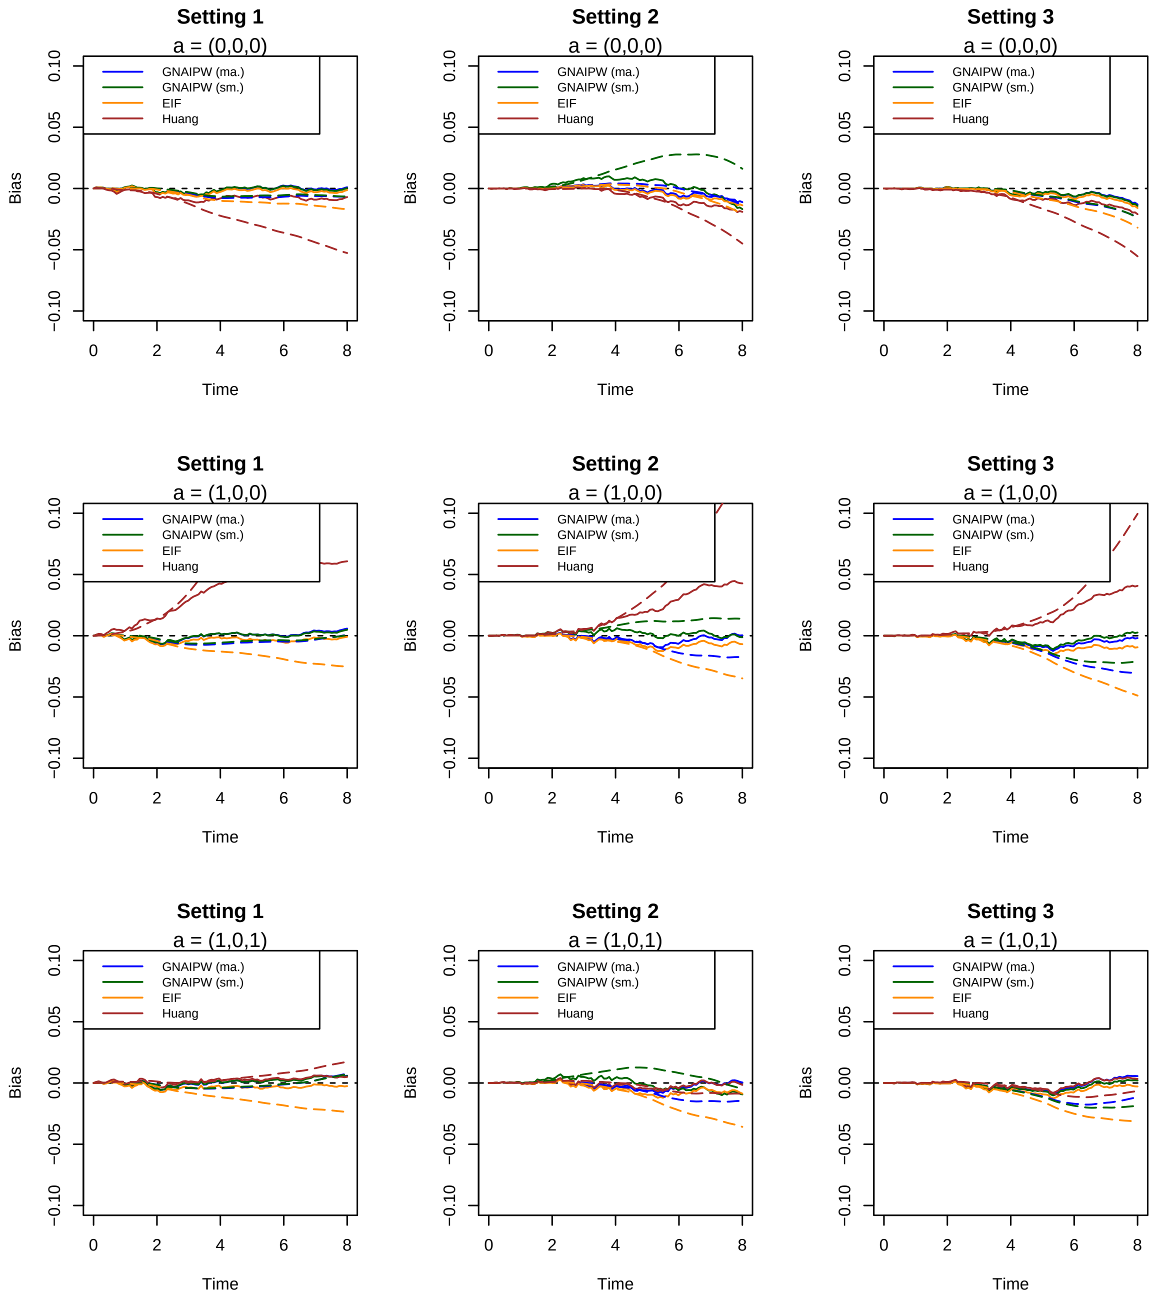


Figure S8: Pointwise bias (solid lines) of estimated cumulative incidences and RMST (dashed lines) by the GNAIPW (Markov), GNAIPW (semi-Markov), EIF-based estimator, and Huang (2021)'s method when $n = 500$.

$F^{(0,0,0)}(t)$, $F^{(1,0,0)}(t)$, and $F^{(1,0,1)}(t)$, respectively. The confidence intervals perform well when the sample size is large enough. When all models and assumptions are correctly specified, the coverage rate of the confidence interval is close to the nominal level. At the tail (when $t$ is large), the number of remaining at-risk individuals is small, so the estimation hashigh variation and the confidence interval is not very stable. The EIF-based estimator presumes Markovness. When Markovness fails, the asymptotic variance of the EIF-based estimator calculted from the plugged-in influence function is incorrect. Therefore, the confidence interval by the EIF-based method may yield an incorrect coverage rate in Setting 3.

## H.3 Empirical type I error rate and power for hypothesis tests

We examine the performance of hypothesis tests on $H_0^1$, $H_0^2$ and $H_0^3$. In each setting, we consider six scenarios where (a) $\emptyset$, (b) $\{H_0^1\}$, (c) $\{H_0^2\}$, (d) $\{H_0^3\}$, (e) $\{H_0^2, H_0^3\}$, and (f) $\{H_0^1, H_0^2, H_0^3\}$ hold(s), respectively. The data generating process is identical to that in Simulation Section except that we set the treatment effect on the $j$th hazard to be null if $H_0^j$ should be satisfied, $j = 1, 2, 3$.

We set the significance level at 0.05. The empirical type I error rate (power) is calculated as the frequency of rejecting the null hypothesis in 10000 independently generated datasets, as shown in Table S4. The cells in bold font type refer to the scenarios where the null hypothesis holds and the assumption (Markov or semi-Markov) on $d\Lambda^{a_3}(t; r)$ is correctly specified, so these empirical type I error rates should be close to 0.05. Although we use estimated propensity score instead of true propensity score, the empirical type I error rate is still close to the nominal level. We observe slight deviation of the empirical type I error rate from 0.05 when the assumption on $d\Lambda^{a_3}(t; r)$ is misspecified. When the sample size is larger, the power becomes larger under the alternative hypothesis.

## H.4 Simulation in the general case

Suppose that covariates are not isolated in these three hazards. The additive hazards models are replaced with proportional hazards models as follows.

1. Setting 1: $d\Lambda_1^a(t; x) = 0.15(x_1 + a)dt$, $d\Lambda_2^a(t; x) = 0.1(x_1 + a)dt$, $d\Lambda_3^a(t; x) = 0.2(x_1 + a)dt$.
2. Setting 2: $d\Lambda_1^a(t; x) = 0.04(x_1 + a)tdt$, $d\Lambda_2^a(t; x) = 0.02(x_1 + a)tdt$, $d\Lambda_3^a(t; x) = 0.05(x_1 + a)tdt$.
3. Setting 3: $d\Lambda_1^a(t; x) = 0.04(x_1 + a)tdt$, $d\Lambda_2^a(t; x) = 0.02(x_1 + a)tdt$, $d\Lambda_3^a(t; r, x) = 0.1(x_1 + a)(t - r)dt$.

There is a common covariate $X_1$ that has an effect on all hazards. Assumption 5 fails but Assumption 8 holds.

Figure S9 showw the pointwise bias of estimated cumulative incidences and RMST in these three settings. The bias when estimating $F^{(0,0,0)}(t)$ is negligible because the treatment combination $A_1 = A_2 = A_3 = 0$ is observable in the realized trial. The bias when estimating $F^{(1,0,0)}(t)$ and $F^{(1,0,1)}(t)$ may depends on specific data generating structures. In our simulation, the bias of GNAIPW is small. The proposed method using Markov assumption is more robust than those using semi-Markov assumption and Huang (2021)'s method.

## H.5 Sensitivity analysis with interacting treatment components

Suppose that the treatment components have interacting effects on hazards. The components $A_1$ and $A_3$ both have direct effects on the direct terminal event and indirect terminal event. The hazards models are now replaced with proportional hazards models as follows.

Table S1: Coverage rate and width of the 95% confidence intervals for $F^{(0,0,0)}(t)$

| | Size | Method | 1 | 2 | 3 | 4 | 5 | 6 | 7 | 8 |
|---|---|---|---|---|---|---|---|---|---|---|
| Setting 1 (Markov and semi-Markov correct) | | | | | | | | | | |
| Coverage | 100 | ma. | 0.901 | 0.909 | 0.913 | 0.933 | 0.924 | 0.923 | 0.924 | 0.923 |
| Width | | | 0.180 | 0.239 | 0.260 | 0.286 | 0.294 | 0.296 | 0.298 | 0.305 |
| Coverage | | sm. | 0.900 | 0.909 | 0.915 | 0.916 | 0.929 | 0.924 | 0.929 | 0.926 |
| Width | | | 0.179 | 0.235 | 0.263 | 0.279 | 0.286 | 0.289 | 0.293 | 0.299 |
| Coverage | | EIF | 0.896 | 0.903 | 0.905 | 0.924 | 0.920 | 0.918 | 0.914 | 0.921 |
| Width | | | 0.178 | 0.235 | 0.262 | 0.277 | 0.282 | 0.282 | 0.282 | 0.283 |
| Coverage | 500 | ma. | 0.937 | 0.942 | 0.944 | 0.940 | 0.946 | 0.953 | 0.939 | 0.943 |
| Width | | | 0.083 | 0.108 | 0.122 | 0.129 | 0.133 | 0.134 | 0.136 | 0.140 |
| Coverage | | sm. | 0.942 | 0.945 | 0.950 | 0.948 | 0.951 | 0.954 | 0.946 | 0.942 |
| Width | | | 0.082 | 0.105 | 0.117 | 0.125 | 0.129 | 0.130 | 0.132 | 0.136 |
| Coverage | | EIF | 0.939 | 0.944 | 0.942 | 0.938 | 0.947 | 0.955 | 0.945 | 0.942 |
| Width | | | 0.083 | 0.108 | 0.121 | 0.128 | 0.132 | 0.132 | 0.133 | 0.137 |
| Setting 2 (Markov correct) | | | | | | | | | | |
| Coverage | 100 | ma. | 0.444 | 0.879 | 0.898 | 0.922 | 0.929 | 0.939 | 0.926 | 0.918 |
| Width | | | 0.046 | 0.126 | 0.192 | 0.241 | 0.274 | 0.292 | 0.302 | 0.312 |
| Coverage | | sm. | 0.446 | 0.88 | 0.905 | 0.926 | 0.935 | 0.941 | 0.933 | 0.914 |
| Width | | | 0.0469 | 0.128 | 0.193 | 0.240 | 0.272 | 0.288 | 0.298 | 0.309 |
| Coverage | | EIF | 0.552 | 0.863 | 0.889 | 0.915 | 0.922 | 0.932 | 0.916 | 0.886 |
| Width | | | 0.154 | 0.126 | 0.190 | 0.237 | 0.268 | 0.282 | 0.287 | 0.290 |
| Coverage | 500 | ma. | 0.897 | 0.930 | 0.939 | 0.945 | 0.946 | 0.949 | 0.940 | 0.934 |
| Width | | | 0.031 | 0.062 | 0.089 | 0.110 | 0.124 | 0.132 | 0.137 | 0.145 |
| Coverage | | sm. | 0.900 | 0.931 | 0.931 | 0.936 | 0.933 | 0.956 | 0.946 | 0.925 |
| Width | | | 0.031 | 0.062 | 0.089 | 0.108 | 0.121 | 0.129 | 0.133 | 0.139 |
| Coverage | | EIF | 0.892 | 0.932 | 0.939 | 0.946 | 0.947 | 0.946 | 0.934 | 0.931 |
| Width | | | 0.032 | 0.063 | 0.090 | 0.110 | 0.124 | 0.131 | 0.135 | 0.142 |
| Setting 3 (semi-Markov correct) | | | | | | | | | | |
| Coverage | 100 | ma. | 0.425 | 0.889 | 0.897 | 0.907 | 0.943 | 0.927 | 0.930 | 0.921 |
| Width | | | 0.044 | 0.127 | 0.191 | 0.239 | 0.272 | 0.289 | 0.300 | 0.313 |
| Coverage | | sm. | 0.426 | 0.89 | 0.901 | 0.91 | 0.937 | 0.934 | 0.925 | 0.927 |
| Width | | | 0.045 | 0.128 | 0.191 | 0.237 | 0.269 | 0.286 | 0.298 | 0.312 |
| Coverage | | EIF | 0.543 | 0.879 | 0.891 | 0.897 | 0.935 | 0.921 | 0.923 | 0.910 |
| Width | | | 0.161 | 0.126 | 0.189 | 0.234 | 0.265 | 0.279 | 0.287 | 0.293 |
| Coverage | 500 | ma. | 0.89 | 0.937 | 0.941 | 0.942 | 0.947 | 0.943 | 0.947 | 0.923 |
| Width | | | 0.030 | 0.062 | 0.089 | 0.109 | 0.123 | 0.131 | 0.137 | 0.146 |
| Coverage | | sm. | 0.890 | 0.938 | 0.939 | 0.937 | 0.944 | 0.941 | 0.943 | 0.927 |
| Width | | | 0.030 | 0.062 | 0.088 | 0.107 | 0.121 | 0.128 | 0.134 | 0.141 |
| Coverage | | EIF | 0.882 | 0.942 | 0.943 | 0.943 | 0.945 | 0.939 | 0.946 | 0.908 |
| Width | | | 0.031 | 0.063 | 0.089 | 0.109 | 0.123 | 0.130 | 0.136 | 0.143 |

Table S2: Coverage rate and width of the 95% confidence intervals for $F^{(1,0,0)}(t)$

| | Size | Method | 1 | 2 | 3 | 4 | 5 | 6 | 7 | 8 |
|---|---|---|---|---|---|---|---|---|---|---|
| Setting 1 (Markov and semi-Markov correct) | | | | | | | | | | |
| Coverage | 100 | ma. | 0.929 | 0.937 | 0.941 | 0.933 | 0.925 | 0.921 | 0.890 | 0.886 |
| Width | | | 0.215 | 0.253 | 0.259 | 0.251 | 0.236 | 0.218 | 0.202 | 0.192 |
| Coverage | | sm. | 0.930 | 0.938 | 0.944 | 0.935 | 0.931 | 0.932 | 0.918 | 0.908 |
| Width | | | 0.215 | 0.252 | 0.257 | 0.248 | 0.233 | 0.216 | 0.203 | 0.197 |
| Coverage | | EIF | 0.931 | 0.929 | 0.947 | 0.940 | 0.947 | 0.936 | 0.947 | 0.940 |
| Width | | | 0.212 | 0.248 | 0.252 | 0.242 | 0.227 | 0.209 | 0.193 | 0.181 |
| Coverage | 500 | ma. | 0.953 | 0.949 | 0.94 | 0.939 | 0.943 | 0.937 | 0.933 | 0.927 |
| Width | | | 0.097 | 0.114 | 0.117 | 0.114 | 0.108 | 0.101 | 0.095 | 0.091 |
| Coverage | | sm. | 0.952 | 0.945 | 0.941 | 0.942 | 0.945 | 0.945 | 0.930 | 0.924 |
| Width | | | 0.097 | 0.112 | 0.114 | 0.111 | 0.105 | 0.098 | 0.093 | 0.091 |
| Coverage | | EIF | 0.955 | 0.950 | 0.938 | 0.936 | 0.946 | 0.927 | 0.927 | 0.927 |
| Width | | | 0.097 | 0.113 | 0.115 | 0.112 | 0.105 | 0.098 | 0.091 | 0.088 |
| Setting 2 (Markov correct) | | | | | | | | | | |
| Coverage | 100 | ma. | 0.847 | 0.919 | 0.928 | 0.933 | 0.931 | 0.928 | 0.894 | 0.865 |
| Width | | | 0.083 | 0.171 | 0.228 | 0.255 | 0.255 | 0.236 | 0.209 | 0.184 |
| Coverage | | sm. | 0.845 | 0.925 | 0.933 | 0.930 | 0.921 | 0.931 | 0.904 | 0.881 |
| Width | | | 0.084 | 0.173 | 0.229 | 0.255 | 0.254 | 0.235 | 0.211 | 0.191 |
| Coverage | | EIF | 0.891 | 0.918 | 0.927 | 0.934 | 0.929 | 0.929 | 0.922 | 0.899 |
| Width | | | 0.123 | 0.170 | 0.225 | 0.250 | 0.249 | 0.228 | 0.201 | 0.174 |
| Coverage | 500 | ma. | 0.942 | 0.939 | 0.957 | 0.947 | 0.942 | 0.944 | 0.939 | 0.934 |
| Width | | | 0.042 | 0.078 | 0.103 | 0.115 | 0.116 | 0.108 | 0.098 | 0.090 |
| Coverage | | sm. | 0.945 | 0.928 | 0.954 | 0.940 | 0.915 | 0.937 | 0.933 | 0.935 |
| Width | | | 0.042 | 0.078 | 0.102 | 0.113 | 0.113 | 0.105 | 0.095 | 0.087 |
| Coverage | | EIF | 0.944 | 0.939 | 0.958 | 0.945 | 0.943 | 0.942 | 0.940 | 0.935 |
| Width | | | 0.042 | 0.078 | 0.102 | 0.114 | 0.114 | 0.106 | 0.095 | 0.087 |
| Setting 3 (semi-Markov correct) | | | | | | | | | | |
| Coverage | 100 | ma. | 0.860 | 0.924 | 0.940 | 0.935 | 0.945 | 0.935 | 0.887 | 0.878 |
| Width | | | 0.084 | 0.170 | 0.227 | 0.255 | 0.256 | 0.239 | 0.214 | 0.193 |
| Coverage | | sm. | 0.861 | 0.929 | 0.946 | 0.938 | 0.938 | 0.935 | 0.896 | 0.884 |
| Width | | | 0.085 | 0.172 | 0.229 | 0.256 | 0.257 | 0.239 | 0.216 | 0.197 |
| Coverage | | EIF | 0.902 | 0.918 | 0.938 | 0.939 | 0.928 | 0.930 | 0.913 | 0.896 |
| Width | | | 0.124 | 0.168 | 0.224 | 0.249 | 0.248 | 0.228 | 0.201 | 0.177 |
| Coverage | 500 | ma. | 0.944 | 0.934 | 0.942 | 0.945 | 0.948 | 0.952 | 0.943 | 0.948 |
| Width | | | 0.041 | 0.078 | 0.103 | 0.115 | 0.116 | 0.110 | 0.101 | 0.094 |
| Coverage | | sm. | 0.944 | 0.934 | 0.935 | 0.944 | 0.951 | 0.961 | 0.931 | 0.940 |
| Width | | | 0.042 | 0.078 | 0.102 | 0.114 | 0.114 | 0.107 | 0.098 | 0.091 |
| Coverage | | EIF | 0.943 | 0.935 | 0.942 | 0.940 | 0.945 | 0.940 | 0.926 | 0.917 |
| Width | | | 0.041 | 0.077 | 0.102 | 0.114 | 0.114 | 0.106 | 0.095 | 0.088 |

Table S3: Coverage rate and width of the 95% confidence intervals for $F^{(1,0,1)}(t)$

| | Size | Method | 1 | 2 | 3 | 4 | 5 | 6 | 7 | 8 |
|---|---|---|---|---|---|---|---|---|---|---|
| Setting 1 (Markov and semi-Markov correct) | | | | | | | | | | |
| Coverage | 100 | ma. | 0.930 | 0.934 | 0.946 | 0.928 | 0.918 | 0.923 | 0.881 | 0.864 |
| Width | | | 0.217 | 0.256 | 0.260 | 0.247 | 0.226 | 0.202 | 0.181 | 0.166 |
| Coverage | | sm. | 0.930 | 0.943 | 0.946 | 0.933 | 0.915 | 0.923 | 0.890 | 0.873 |
| Width | | | 0.216 | 0.252 | 0.255 | 0.242 | 0.222 | 0.199 | 0.180 | 0.169 |
| Coverage | | EIF | 0.932 | 0.932 | 0.947 | 0.937 | 0.944 | 0.935 | 0.925 | 0.910 |
| Width | | | 0.217 | 0.258 | 0.264 | 0.253 | 0.232 | 0.209 | 0.186 | 0.164 |
| Coverage | 500 | ma. | 0.946 | 0.939 | 0.947 | 0.944 | 0.947 | 0.939 | 0.933 | 0.920 |
| Width | | | 0.098 | 0.115 | 0.116 | 0.111 | 0.102 | 0.093 | 0.084 | 0.080 |
| Coverage | | sm. | 0.942 | 0.937 | 0.943 | 0.942 | 0.948 | 0.946 | 0.921 | 0.928 |
| Width | | | 0.097 | 0.112 | 0.113 | 0.107 | 0.099 | 0.090 | 0.082 | 0.076 |
| Coverage | | EIF | 0.944 | 0.945 | 0.956 | 0.951 | 0.955 | 0.960 | 0.957 | 0.958 |
| Width | | | 0.098 | 0.115 | 0.117 | 0.113 | 0.105 | 0.097 | 0.090 | 0.086 |
| Setting 2 (Markov correct) | | | | | | | | | | |
| Coverage | 100 | ma. | 0.847 | 0.920 | 0.927 | 0.926 | 0.923 | 0.929 | 0.888 | 0.825 |
| Width | | | 0.083 | 0.172 | 0.229 | 0.256 | 0.255 | 0.231 | 0.196 | 0.163 |
| Coverage | | sm. | 0.847 | 0.928 | 0.935 | 0.930 | 0.926 | 0.942 | 0.910 | 0.891 |
| Width | | | 0.084 | 0.174 | 0.231 | 0.256 | 0.252 | 0.229 | 0.199 | 0.172 |
| Coverage | | EIF | 0.890 | 0.920 | 0.923 | 0.926 | 0.926 | 0.929 | 0.909 | 0.888 |
| Width | | | 0.123 | 0.171 | 0.232 | 0.260 | 0.260 | 0.237 | 0.200 | 0.157 |
| Coverage | 500 | ma. | 0.943 | 0.941 | 0.961 | 0.939 | 0.937 | 0.939 | 0.942 | 0.925 |
| Width | | | 0.042 | 0.078 | 0.104 | 0.116 | 0.115 | 0.105 | 0.092 | 0.080 |
| Coverage | | sm. | 0.942 | 0.925 | 0.952 | 0.935 | 0.924 | 0.951 | 0.955 | 0.920 |
| Width | | | 0.042 | 0.078 | 0.103 | 0.113 | 0.112 | 0.102 | 0.089 | 0.078 |
| Coverage | | EIF | 0.941 | 0.947 | 0.961 | 0.939 | 0.944 | 0.944 | 0.953 | 0.944 |
| Width | | | 0.042 | 0.078 | 0.104 | 0.116 | 0.116 | 0.107 | 0.096 | 0.087 |
| Setting 3 (semi-Markov correct) | | | | | | | | | | |
| Coverage | 100 | ma. | 0.860 | 0.923 | 0.937 | 0.932 | 0.930 | 0.925 | 0.869 | 0.834 |
| Width | | | 0.084 | 0.170 | 0.227 | 0.256 | 0.256 | 0.237 | 0.207 | 0.179 |
| Coverage | | sm. | 0.861 | 0.930 | 0.939 | 0.942 | 0.944 | 0.934 | 0.897 | 0.871 |
| Width | | | 0.085 | 0.172 | 0.229 | 0.256 | 0.255 | 0.235 | 0.206 | 0.183 |
| Coverage | | EIF | 0.903 | 0.920 | 0.933 | 0.925 | 0.931 | 0.918 | 0.905 | 0.886 |
| Width | | | 0.124 | 0.168 | 0.226 | 0.255 | 0.258 | 0.243 | 0.220 | 0.190 |
| Coverage | 500 | ma. | 0.941 | 0.936 | 0.938 | 0.944 | 0.945 | 0.954 | 0.923 | 0.916 |
| Width | | | 0.041 | 0.078 | 0.103 | 0.115 | 0.115 | 0.107 | 0.096 | 0.087 |
| Coverage | | sm. | 0.942 | 0.936 | 0.939 | 0.941 | 0.947 | 0.949 | 0.927 | 0.916 |
| Width | | | 0.041 | 0.078 | 0.102 | 0.113 | 0.113 | 0.104 | 0.093 | 0.082 |
| Coverage | | EIF | 0.940 | 0.939 | 0.936 | 0.948 | 0.948 | 0.956 | 0.946 | 0.946 |
| Width | | | 0.041 | 0.078 | 0.103 | 0.115 | 0.116 | 0.108 | 0.100 | 0.094 |

Table S4: The empirical type I error rate (power) of tests. Tests for $H_0^3$ can be based on Markov (ma.) assumption or semi-Markov (sm.) assumption

| Setting | Hypotheses satisfied | $n=100$ | | | | $n=500$ | | | |
|---|---|---|---|---|---|---|---|---|---|
| | | $H_0^1$ | $H_0^2$ | $H_0^3$ (ma.) | $H_0^3$ (sm.) | $H_0^1$ | $H_0^2$ | $H_0^3$ (ma.) | $H_0^3$ (sm.) |
| 1 | None | 0.858 | 0.698 | 0.450 | 0.470 | 1.000 | 1.000 | 0.990 | 0.992 |
| | $H_0^1$ | **0.045** | 0.787 | 0.490 | 0.483 | **0.044** | 1.000 | 0.994 | 0.9948 |
| | $H_0^2$ | 0.903 | **0.049** | 0.390 | 0.401 | 1.000 | **0.050** | 0.964 | 0.968 |
| | $H_0^3$ | 0.858 | 0.698 | **0.055** | **0.055** | 1.000 | 1.000 | **0.047** | **0.047** |
| | $H_0^2$, $H_0^3$ | 0.903 | **0.049** | **0.055** | **0.055** | 1.000 | **0.050** | **0.052** | **0.051** |
| | All | **0.046** | **0.045** | **0.056** | **0.055** | **0.045** | **0.048** | **0.051** | **0.048** |
| 2 | None | 0.886 | 0.612 | 0.370 | 0.287 | 1.000 | 0.999 | 0.966 | 0.896 |
| | $H_0^1$ | **0.042** | 0.706 | 0.409 | 0.351 | **0.045** | 1.000 | 0.982 | 0.958 |
| | $H_0^2$ | 0.916 | **0.049** | 0.318 | 0.266 | 1.000 | **0.049** | 0.918 | 0.8412 |
| | $H_0^3$ | 0.886 | 0.612 | **0.055** | 0.057 | 1.000 | 0.999 | **0.052** | 0.071 |
| | $H_0^2$, $H_0^3$ | 0.916 | **0.049** | **0.060** | 0.056 | 1.000 | **0.049** | **0.049** | 0.052 |
| | All | **0.043** | **0.048** | **0.055** | 0.055 | **0.044** | **0.046** | **0.051** | 0.051 |
| 3 | None | 0.885 | 0.608 | 0.277 | 0.305 | 1.000 | 0.999 | 0.951 | 0.927 |
| | $H_0^1$ | **0.046** | 0.708 | 0.209 | 0.309 | **0.047** | 1.000 | 0.892 | 0.9394 |
| | $H_0^2$ | 0.920 | **0.049** | 0.217 | 0.264 | 1.000 | **0.047** | 0.830 | 0.845 |
| | $H_0^3$ | 0.885 | 0.608 | 0.043 | **0.058** | 1.000 | 0.999 | 0.072 | **0.051** |
| | $H_0^2$, $H_0^3$ | 0.920 | **0.049** | 0.046 | **0.060** | 1.000 | **0.047** | 0.051 | **0.050** |
| | All | **0.042** | **0.046** | 0.036 | **0.057** | **0.046** | **0.047** | 0.03 | **0.047** |

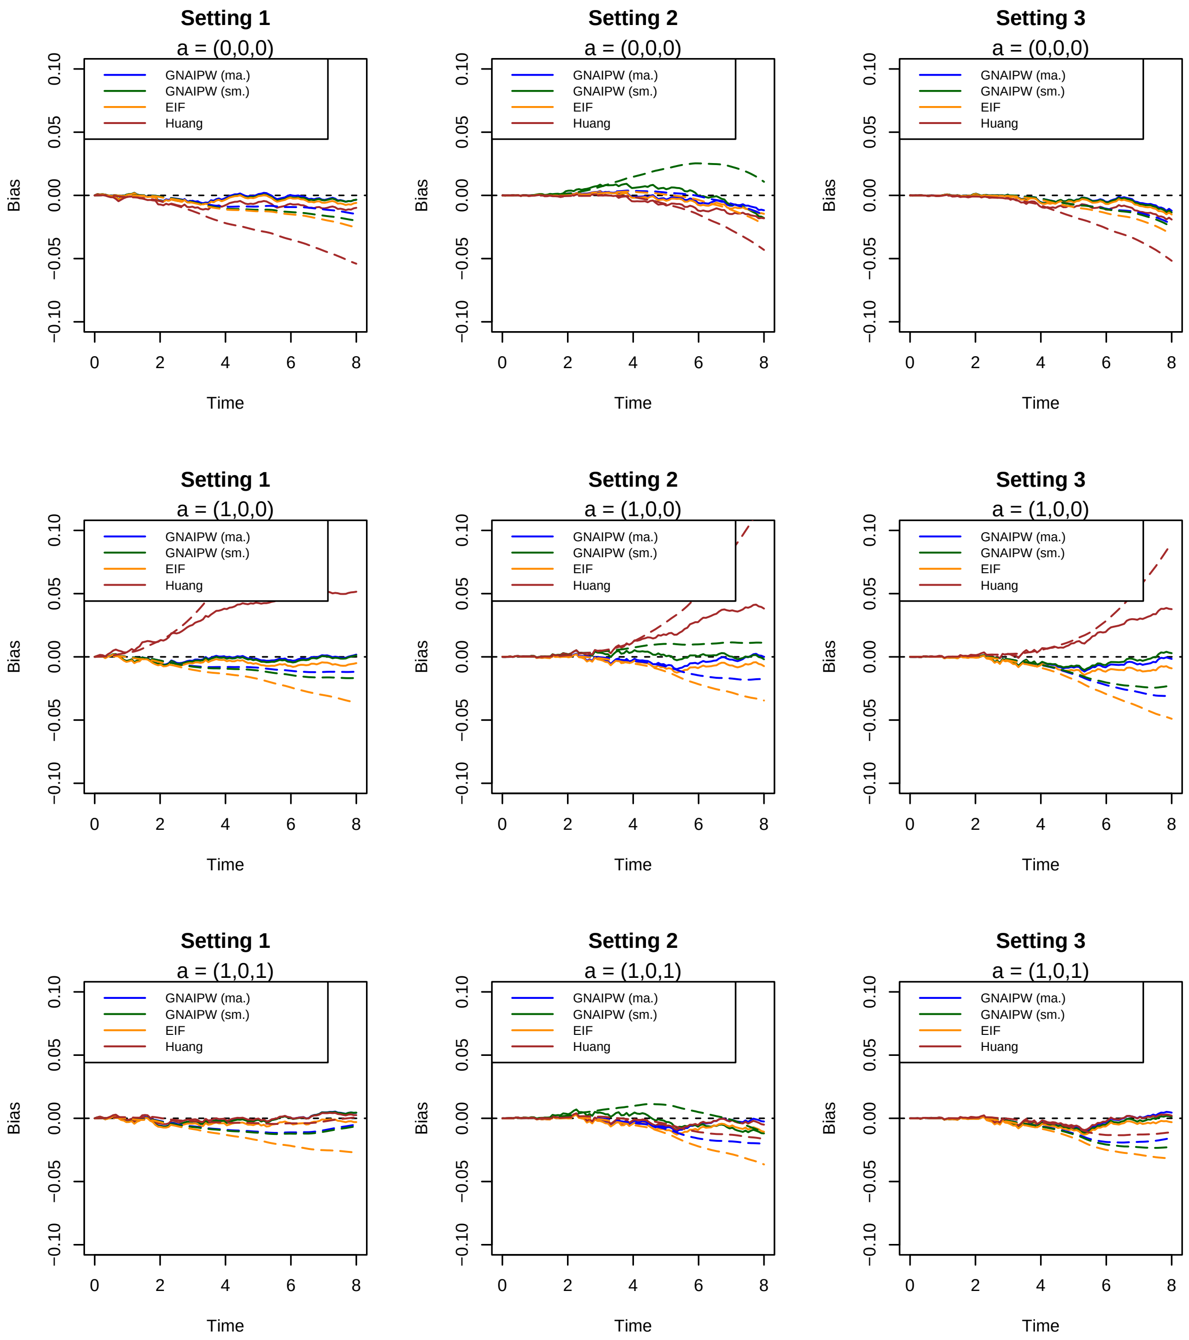


Figure S9: Pointwise bias (solid lines) of estimated cumulative incidences and RMST (dashed lines) in estimating $F^{(0,0,0)}(t)$, $F^{(1,0,0)}(t)$ and $F^{(1,0,1)}(t)$ when $n = 500$. The covariates isolation fails but the conditional dismissible components assumption holds.

1. Setting 1: $d\Lambda_1^a(t;x) = 0.15(x_1 + a_1 + a_3/2)dt$, $d\Lambda_2^a(t;x) = 0.1(x_1 + a_2)dt$, $d\Lambda_3^a(t;x) = 0.2(x_2 + a_3 + a_1/2)dt$.

2. Setting 2: $d\Lambda_1^a(t;x) = 0.04(x_1 + a_1 + a_3/2)tdt$, $d\Lambda_2^a(t;x) = 0.02(x_1 + a_2)tdt$, $d\Lambda_3^a(t;x) = 0.05(x_2 + a_3 + a_1/2)tdt$.

3. Setting 3: $d\Lambda_1^a(t;x) = 0.04(x_1 + a_1 + a_3/2)tdt$, $d\Lambda_2^a(t;x) = 0.02(x_1 + a_2)tdt$, $d\Lambda_3^a(t;r,x) = 0.1(x_2 + a_3 + a_1/2)(t-r)dt$.

In a hypothetical experiment, we can always envision some treatment components that satisfies Assumption 8. However, envisioning groundless treatment components may lose meaningful interpretations. It may be worth studying the bias of the estimators when explanable treatment components have interacting effects.

Figure S10 shows the pointwise bias of estimated cumulative incidences and RMST in these three settings with interacting treatment components. For the proposed methods, the bias is large when estimating the counterfactual $F^{(1,0,0)}(t)$. The bias is negligible when estimating $F^{(0,0,0)}(t)$ and $F^{(1,0,1)}(t)$ since $A_1$ and $A_3$ are at the same value.

# I Additional data analysis results

The first two panels of Figure S11 show the estimated cumulative incidences of mortality by Markovness and semi-Markovness with 95% confidence intervals. The black line is the estimated cumulative incidence of mortality by the generalized Nelson–Aalen estimator which ignores the intermediate event (intention-to-treat analysis). The generalized Nelson–Aalen estimator is consistent, so a reasonable assumption should make the estimated curve close to the generalized Nelson–Aalen estimator. From the first two panels we see that the generalized Nelson–Aalen estimator is very close to the estimated cumulative incidences by both Markovness and semi-Markovness, and is covered by the 95% confidence intervals by both Markovness and semi-Markovness. So both the Markov and semi-Markov assumption could be reasonable.

To assess the sensitivity of the assumption on $d\Lambda_3^{a_3}(t;r)$, we consider the sensitivity analysis

$$d\Lambda_3^{a_3}(t;r) = (1-\kappa)d\Lambda_{3,\text{ma.}}^{a_3}(t) + \kappa d\Lambda_{3,\text{sm.}}^{a_3}(t-r)$$

where $\kappa \in [0,1]$ is a sensitivity parameter. The third panel of Figure S11 displays the estimated treatment effect (difference of the cumulative incidences $F^{(1,1,1)}(t)$ and $F^{(0,0,0)}(t)$) under several choices of sensitivity parameter. The black line is the estimated treatment effect by the generalized Nelson–Aalen estimator (intention-to-treat analysis) which is always consistent. The sensitivity analysis on the treatment effect does not show obvious difference between the results yielded by Markovness and semi-Markovness. Still, both the Markov and semi-Markov assumption could be reasonable.

## References

Breum, M. S., Munch, A., Gerds, T. A., and Martinussen, T. (2024). Estimation of separable direct and indirect effects in a continuous-time illness-death model. *Lifetime Data Analysis*, 30(1):143–180.

Huang, Y.-T. (2021). Causal mediation of semicompeting risks. *Biometrics*, 77(4):1143–1154.

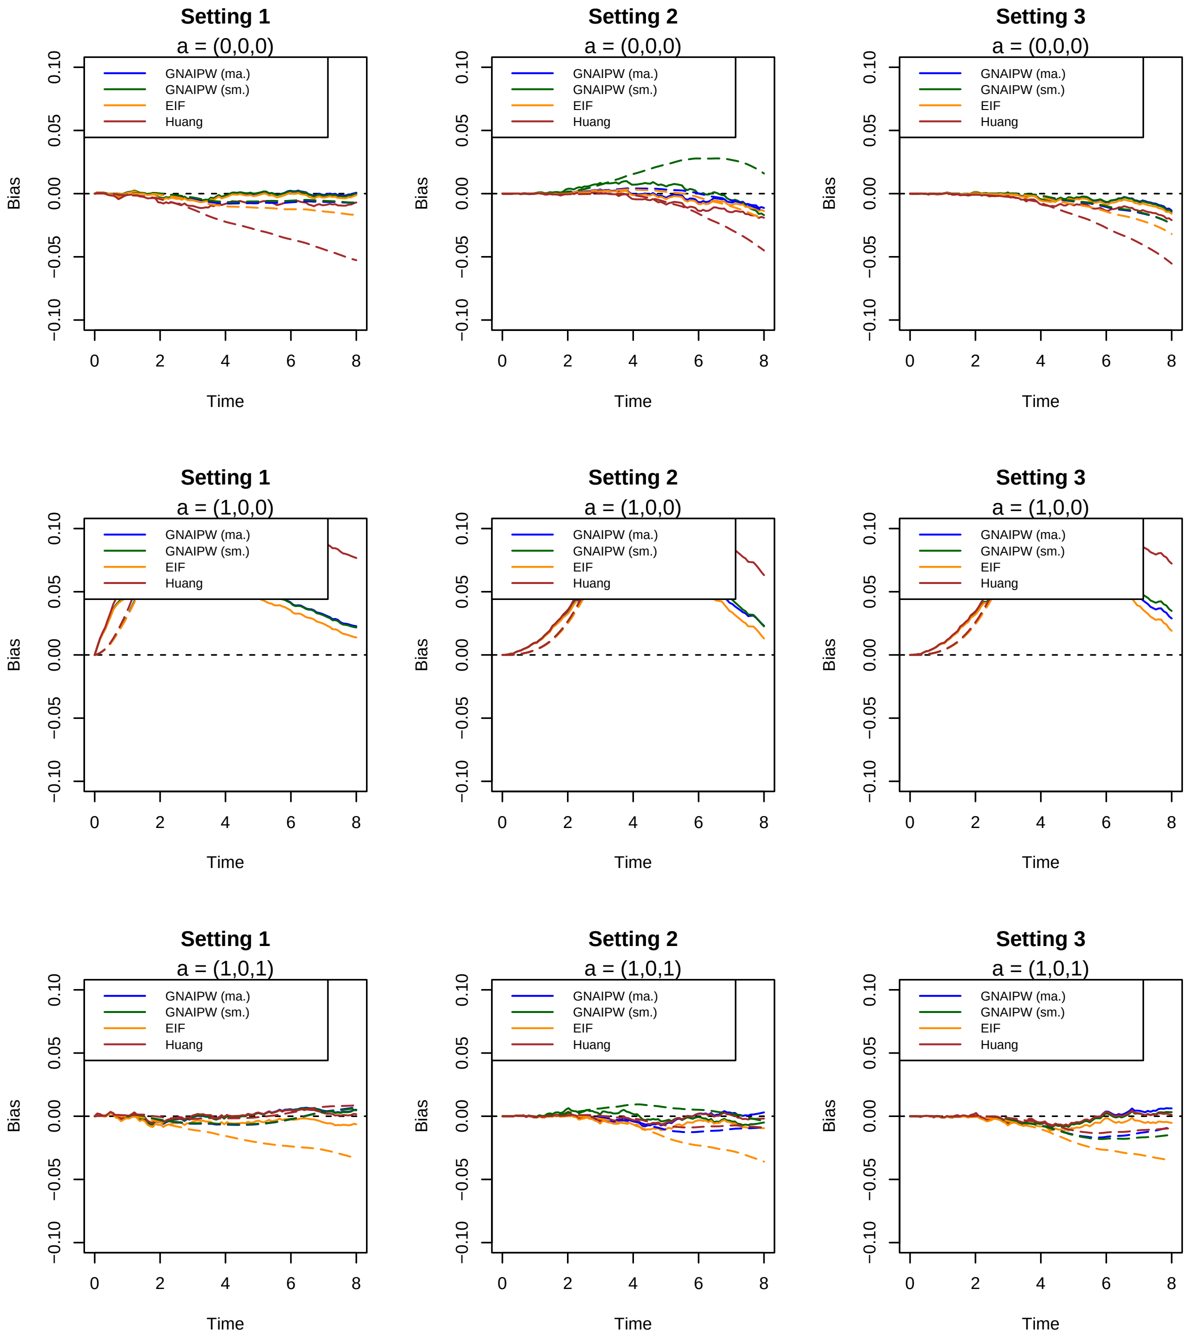


Figure S10: Pointwise bias (solid lines) of estimated cumulative incidences and RMST (dashed lines) in estimating $F^{(0,0,0)}(t)$, $F^{(1,0,0)}(t)$ and $F^{(1,0,1)}(t)$ when $n = 500$. The treatment components have interaction.

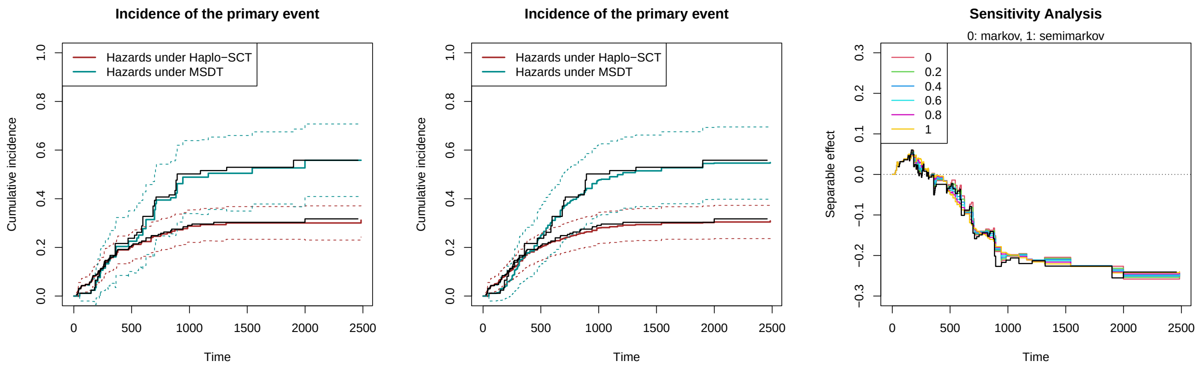


Figure S11: Cumulative incidence of mortality estimated by Markov and semi-Markov, and a sensitivity analysis on the treatment effect. The black line is the estimated curve by generalized Nelson–Aalen estimator ignoring intermediate events.


Huang, Y.-T. (2022). Hypothesis test for causal mediation of time-to-event mediator and outcome. *Statistics in Medicine*, 41(11):1971–1985.

Kalbfleisch, J. D. and Prentice, R. L. (2011). *The statistical analysis of failure time data*. John Wiley & Sons.

Martinussen, T. and Stensrud, M. J. (2023). Estimation of separable direct and indirect effects in continuous time. *Biometrics*, 79(1):127–139.

Robins, J. M. (1997). Causal inference from complex longitudinal data. In *Latent Variable Modeling and Applications to Causality*, pages 69–117. Springer.

Robins, J. M. and Richardson, T. S. (2010). Alternative graphical causal models and the identification of direct effects. *Causality and psychopathology: Finding the determinants of disorders and their cures*, 84:103–158.

Stensrud, M. J., Young, J. G., Didelez, V., Robins, J. M., and Hernán, M. A. (2022). Separable effects for causal inference in the presence of competing events. *Journal of the American Statistical Association*, 117(537):175–183.

Young, J. G., Stensrud, M. J., Tchetgen Tchetgen, E. J., and Hernán, M. A. (2020). A causal framework for classical statistical estimands in failure-time settings with competing events. *Statistics in Medicine*, 39(8):1199–1236.
